# Supplementary material for: A Multi-Labeled Dataset for Indonesian Discourse: Examining Toxicity, Polarization, and Demographics Information
Source: arXiv:2503.00417 source file (2025-03-01)
Supplement: Supplementary file 1 [file divisive_text.tex]

\section{Example of Divisive Texts}
\label{app:divisive-text}

A list of divisive text is available in Table \ref{tab:divisive-text}.

\begin{table*}[ht]
\centering
\small
\begin{tabular}{p{8.5cm}|p{6.5cm}}
\hline
\textbf{Divisive Text} & \textbf{Comment} \\
\hline
Around 800 to 1000 Christians still live in Gaza, which is one of the oldest Christian communities worldwide. They are also evicted and killed. Entire faith groups died out in the land where Christianity originated. & \textbf{3 of 3 Christians or Catholics}, and \textbf{0 of 10 non-Christians or Catholics} annotators annotate this text as hate speech. \\
\hline
Be a woman who is crazy about work. Because there are enough women crazy about boys. Even though people keep seeing us hanging out. & \textbf{1 of 4 undergraduates} and \textbf{3 of 3 high school graduates }annotators annotate this text as hate speech. However, \textbf{2 of 5 females} and \textbf{2 of 3 males} annotators annotate this text as hate speech. \\
\hline
"GANJA(Weed) FOR ALL CEBONG" with all their 45 spirit putting up billboards, they forgot one character and turned it into something completely different... hahahaah, this is what happens when you want to scam people. & \textbf{2 of 3 Ganjar voters (Group 3)}, \textbf{5 of 5 Prabowo voters (Group 2)}, and \textbf{0 of 3 Anies voters (Group 1)} annotate this text as hate speech.\\
\hline
Everybody knows that most PDIP supporters are Christians and that anyone gaining the support of PDIP will also get the support of Christians. However, this chances because of Ganjar Pranowo's stance on banning Israel's soccer team from coming to Indonesia to compete, which makes Christians unhappy. & \textbf{3 of 4 males} and \textbf{0 of 7 females} annotators annotate the text as hate speech. \\
\hline
I used to praise Jokowi but not anymore, why? Because he used his child for evil people. If Gibran was made to become a candidate for president, it would have been okay. But, Gibran was made as a candidate for vice president, used only to gain supporters for Golkar political group. & \textbf{7 of 8 non-Chinese} and \textbf{0 of 3 Chinese} annotators annotate this text as hate speech. \\
\hline
Goooo GaMa (Word play on the president and vice president candidate of Group 3)! Legally defective products will continue to create defective products. & \textbf{6 of 7 Gen Z} and \textbf{0 of 4 Gen X and Millenials} annotate this text as hate speech.\\
\end{tabular}
\caption{Examples of divisive texts and the demographic group in which they are divisive.}
\label{tab:divisive-text}
\vspace{-6pt}
\end{table*}
