# Supplementary material for: A Multi-Labeled Dataset for Indonesian Discourse: Examining Toxicity, Polarization, and Demographics Information
Source: arXiv:2503.00417 source file (2025-03-01)
Supplement: Supplementary file 2 [file heatmaps.tex]

\newpage
\section{Effect of Demographic and Topic Information to Model Performance}
\label{app:heatmaps}

\subsection{gpt-3.5-turbo}
\begin{figure}
    \centering
    \includegraphics[width=1\textwidth]{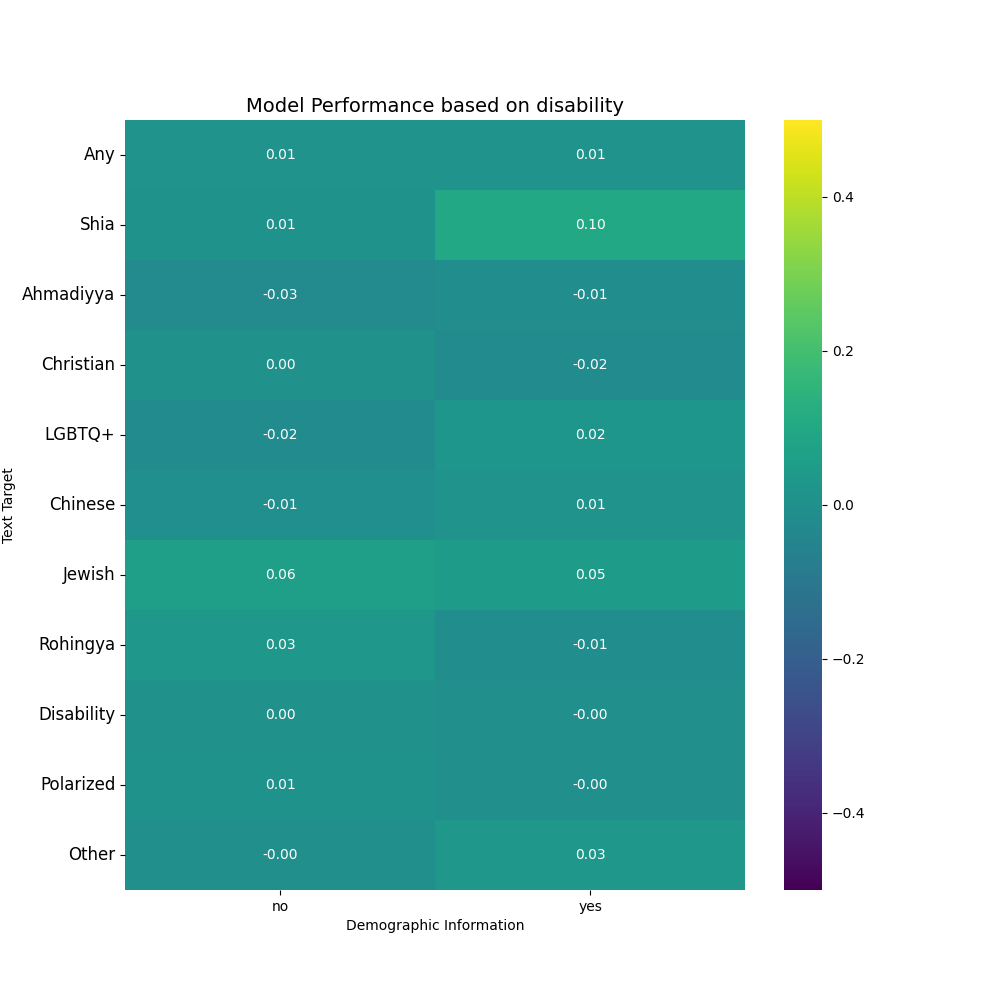}
\end{figure}
\begin{figure}
    \centering
    \includegraphics[width=1\textwidth]{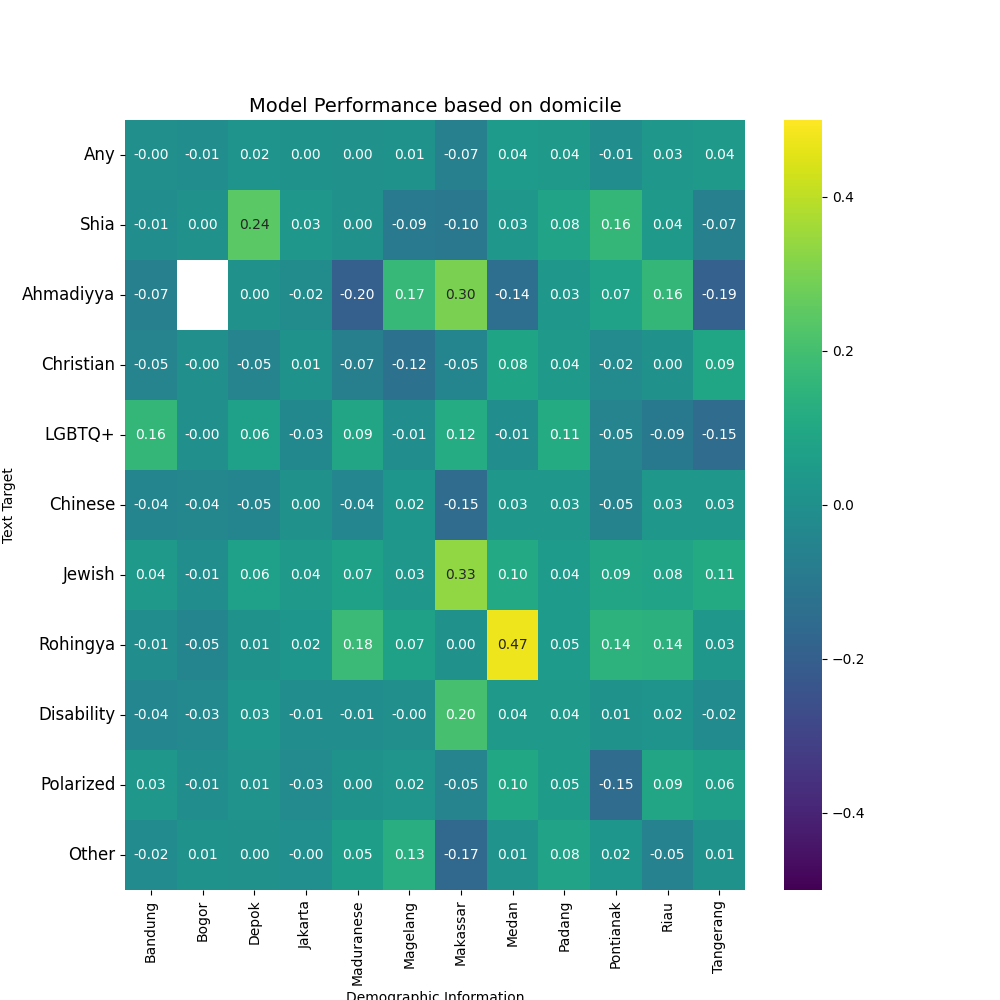}
\end{figure}
\begin{figure}
    \centering
    \includegraphics[width=1\textwidth]{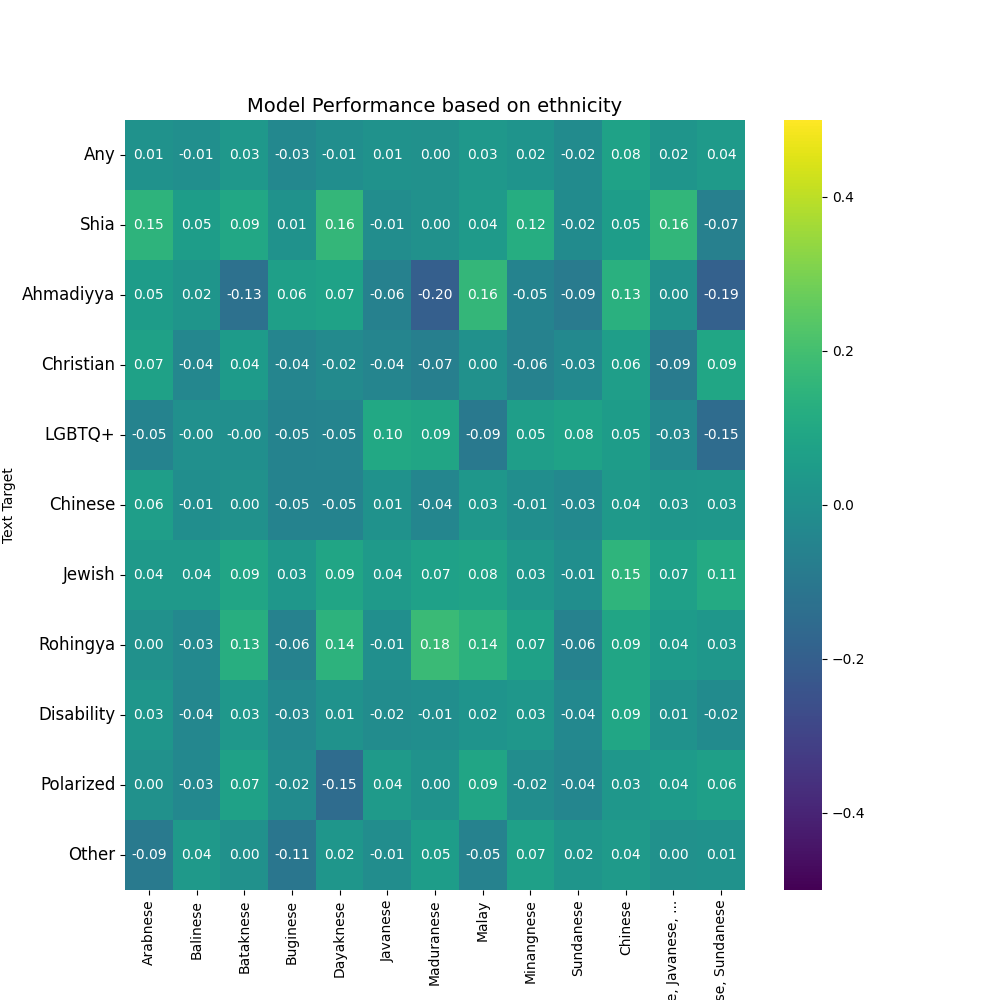}
\end{figure}
\begin{figure}
    \centering
    \includegraphics[width=1\textwidth]{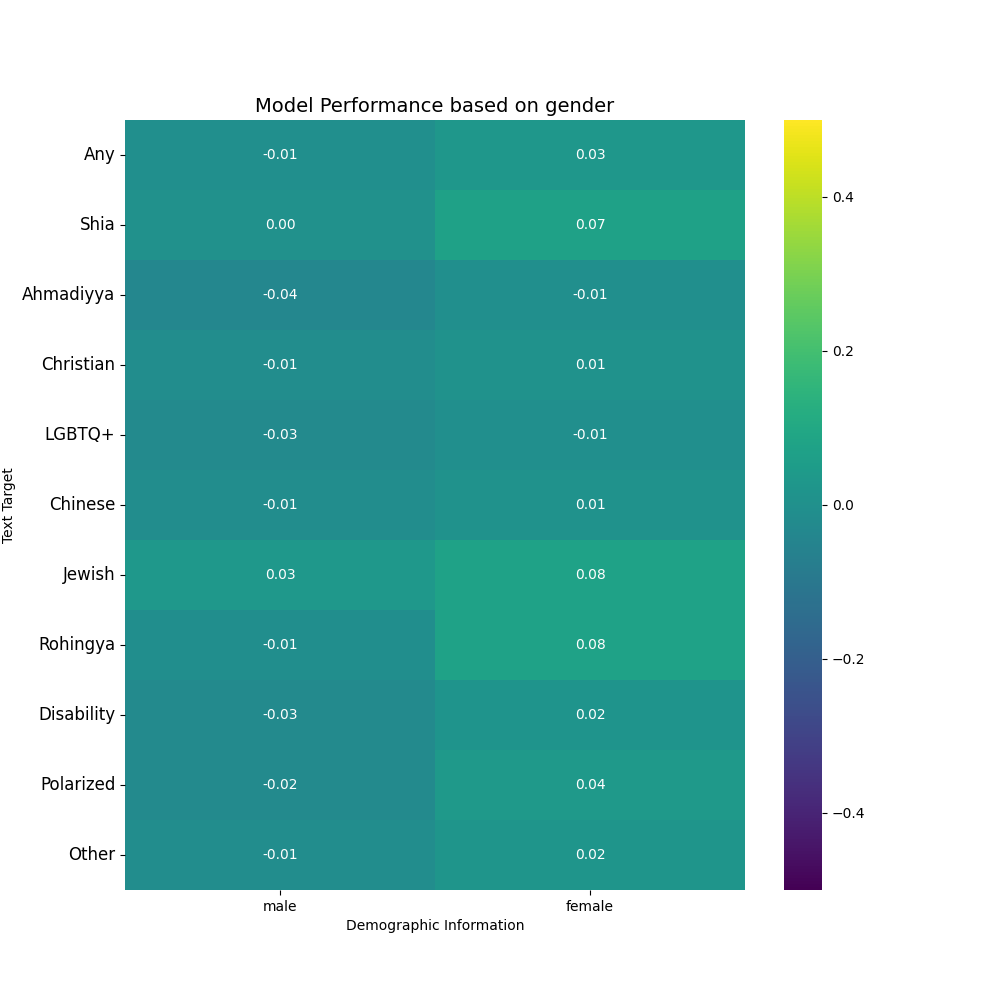}
\end{figure}
\begin{figure}
    \centering
    \includegraphics[width=1\textwidth]{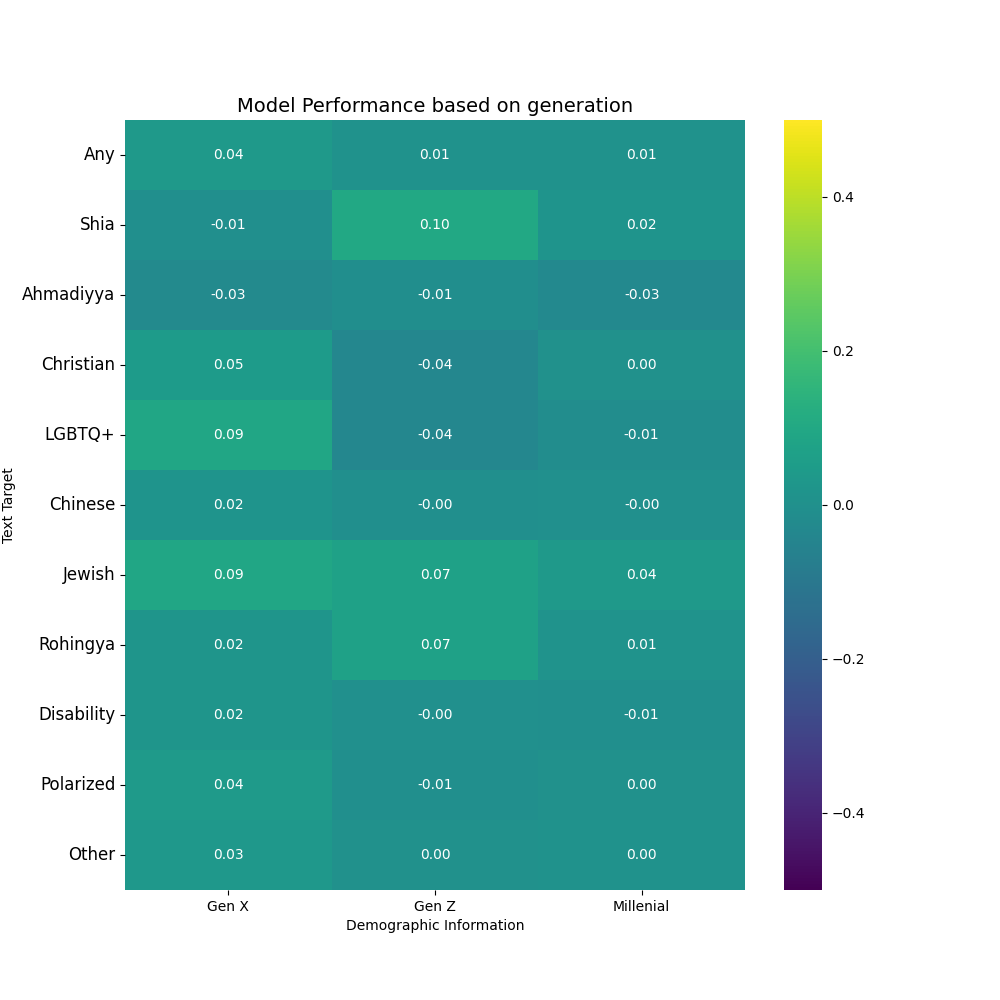}
\end{figure}
\begin{figure}
    \centering
    \includegraphics[width=1\textwidth]{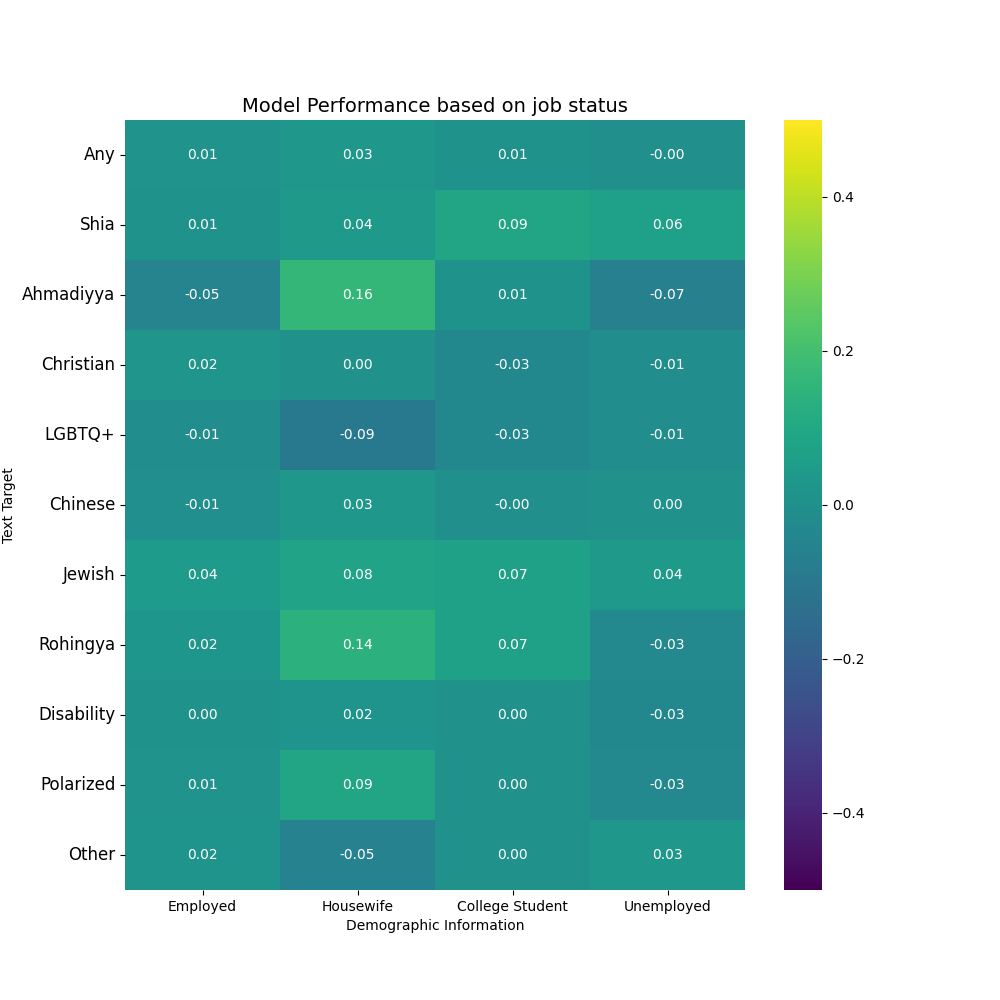}
\end{figure}
\begin{figure}
    \centering
    \includegraphics[width=1\textwidth]{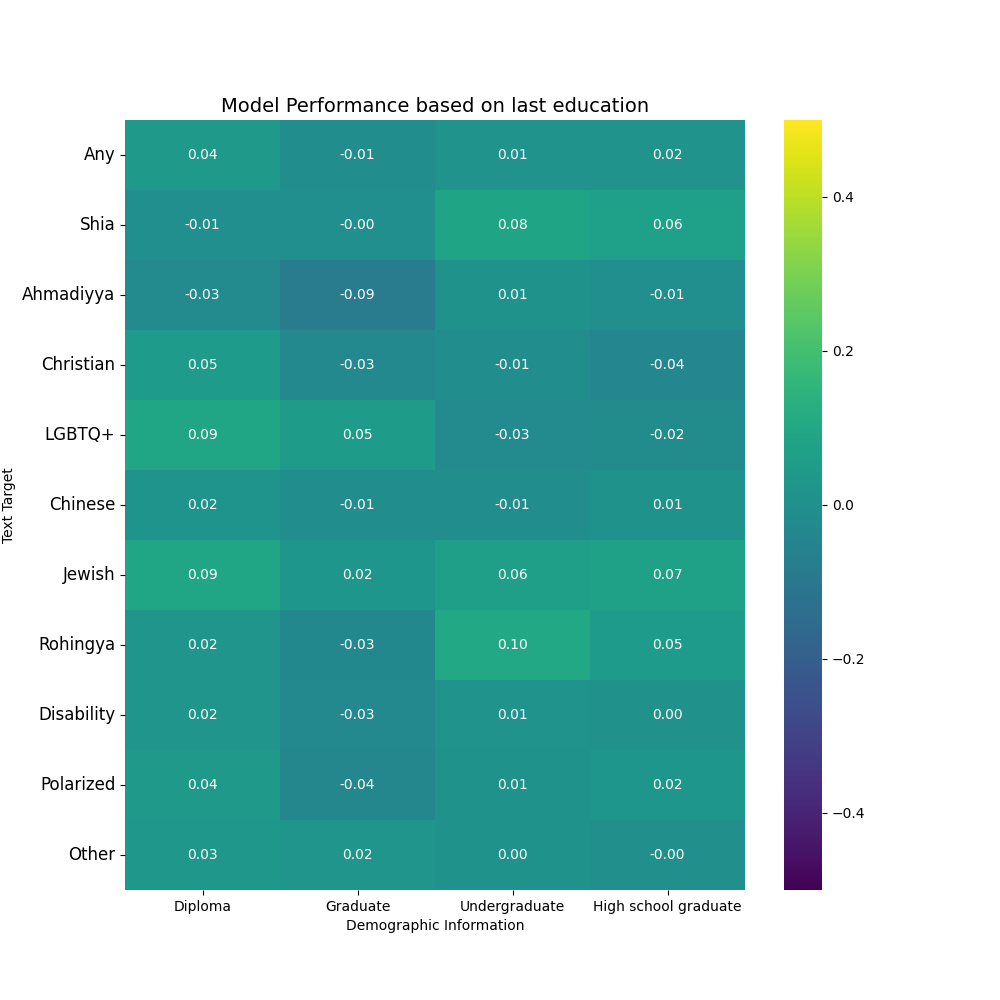}
\end{figure}
\begin{figure}
    \centering
    \includegraphics[width=1\textwidth]{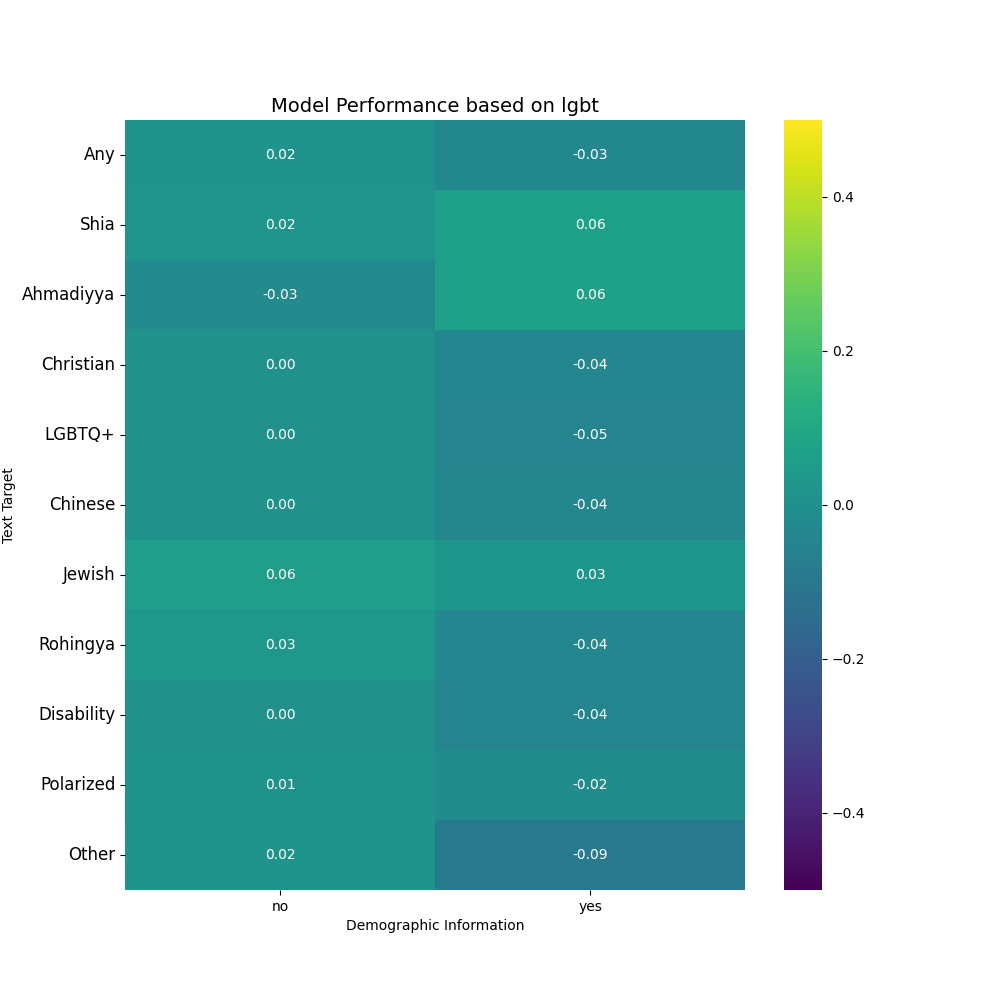}
\end{figure}
\begin{figure}
    \centering
    \includegraphics[width=1\textwidth]{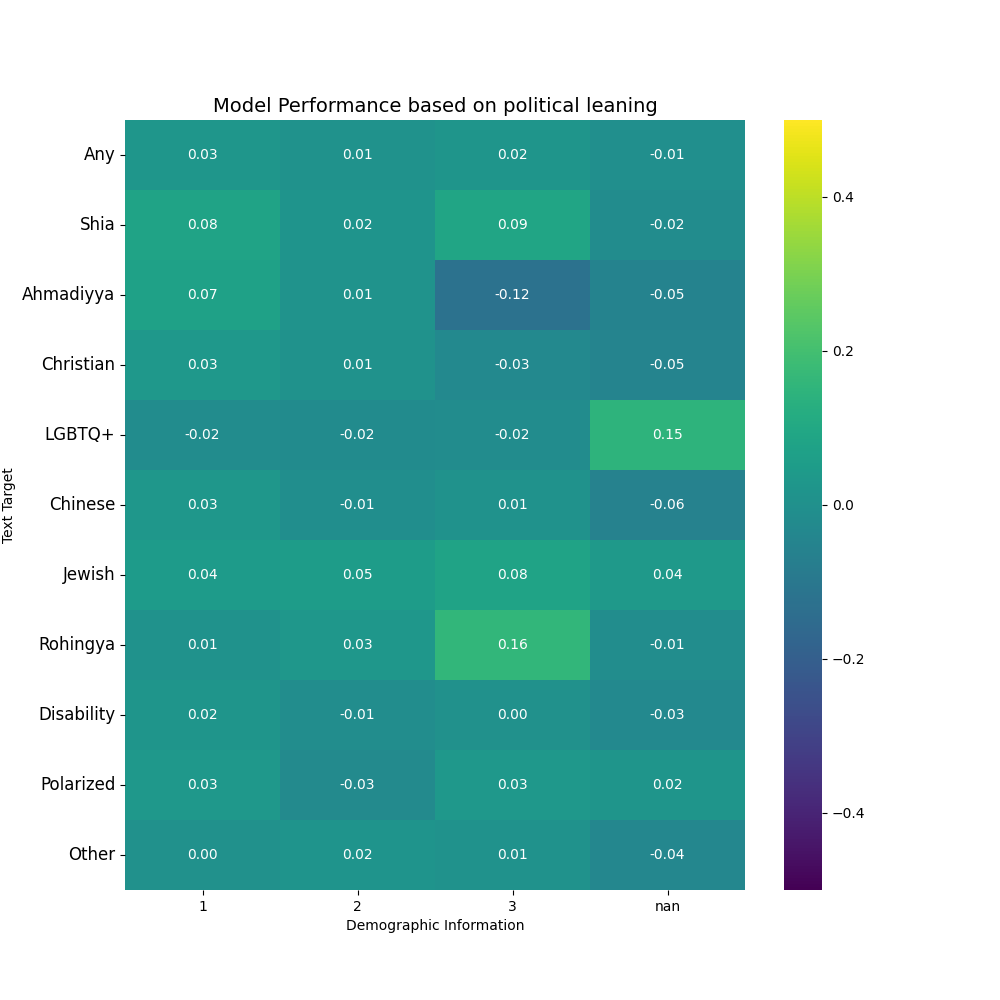}
\end{figure}
\begin{figure}
    \centering
    \includegraphics[width=1\textwidth]{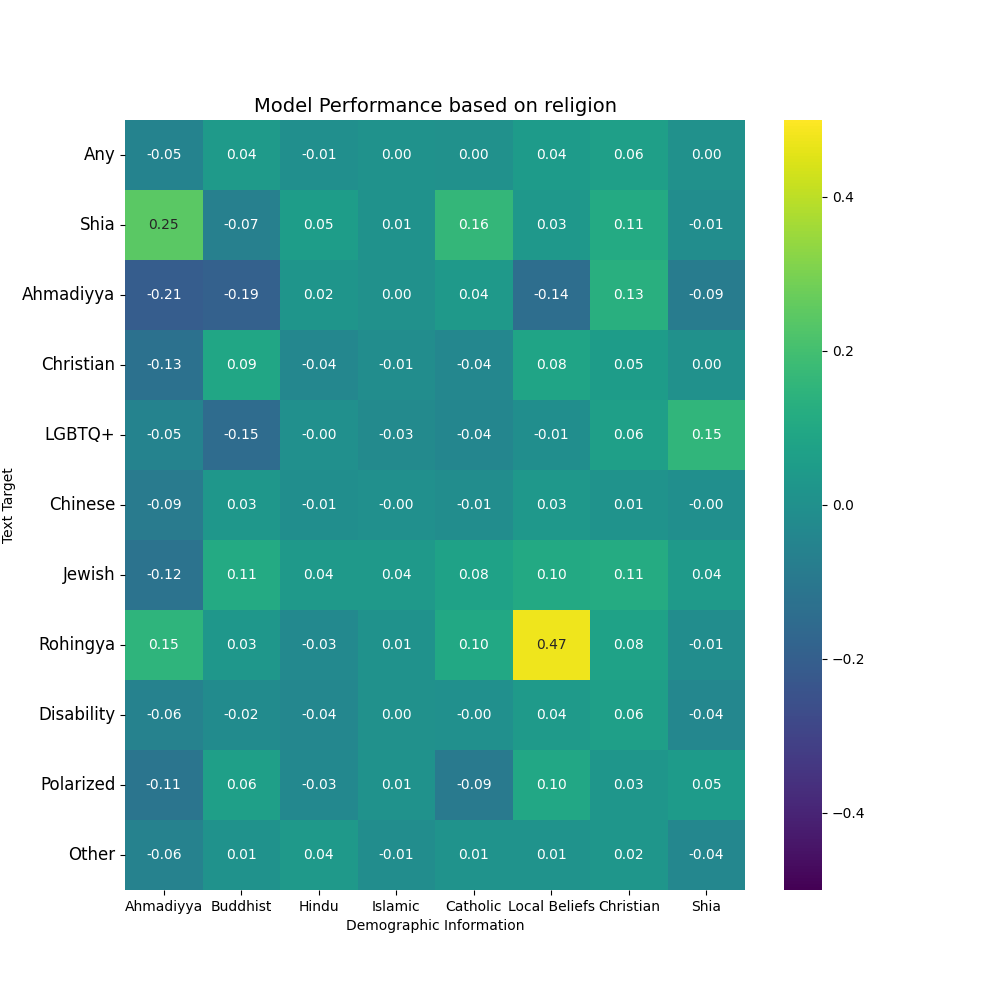}
\end{figure}

\newpage
\subsection{IndoBERTweet with Demographic Information}
\begin{figure}[H]
    \centering
    \includegraphics[width=1\textwidth]{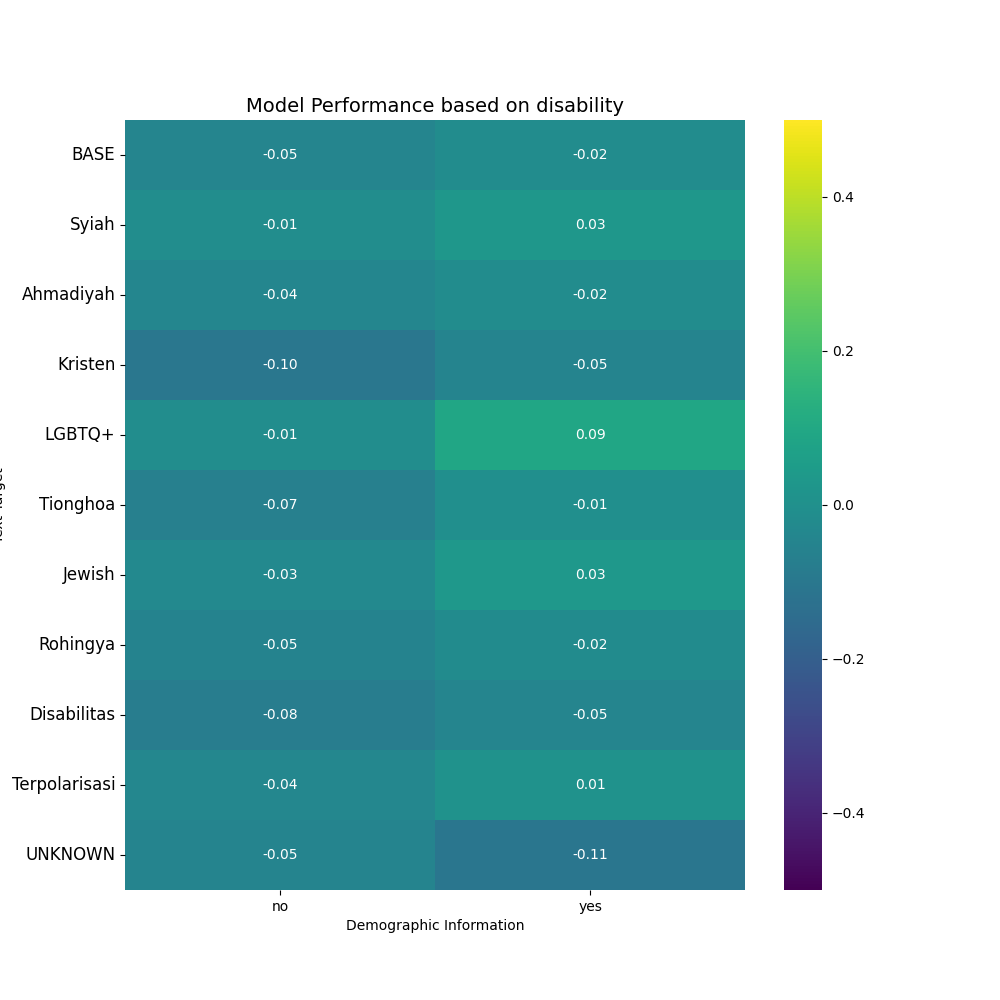}
\end{figure}
\begin{figure}
    \centering
    \includegraphics[width=1\textwidth]{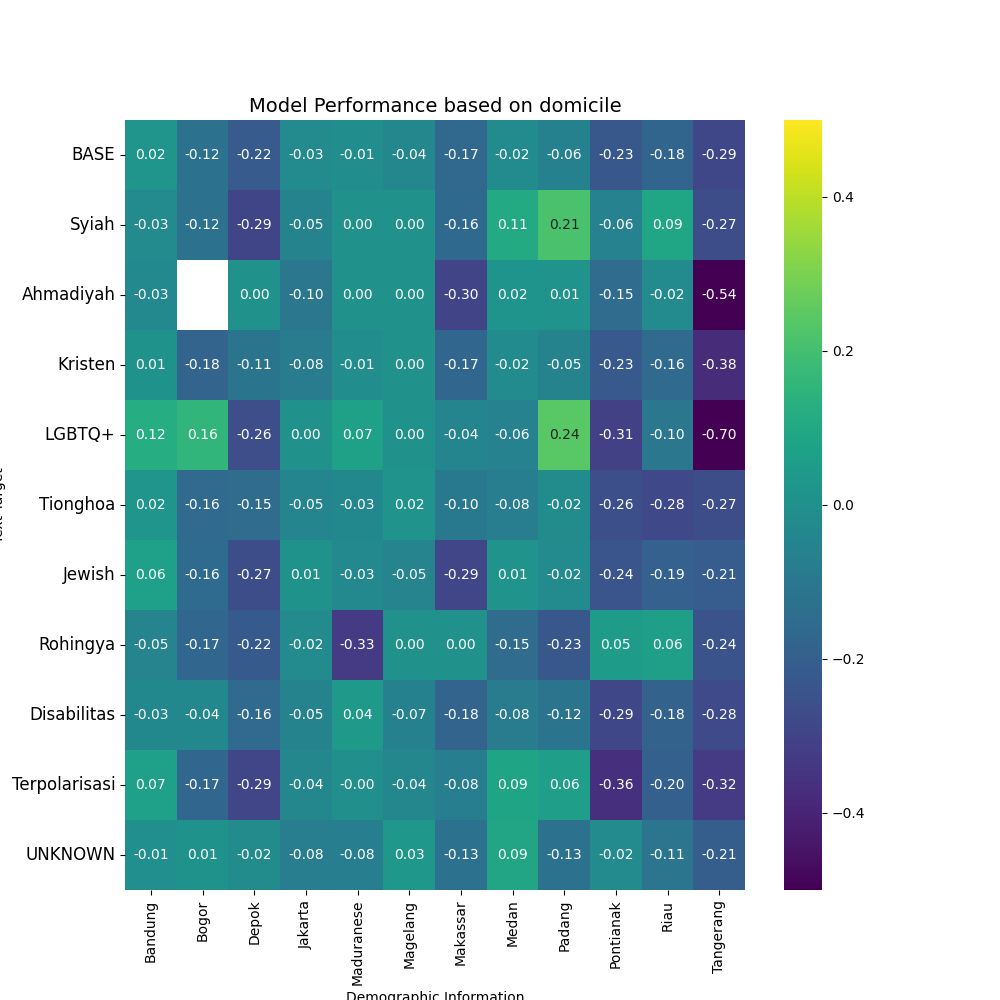}
\end{figure}
\begin{figure}
    \centering
    \includegraphics[width=1\textwidth]{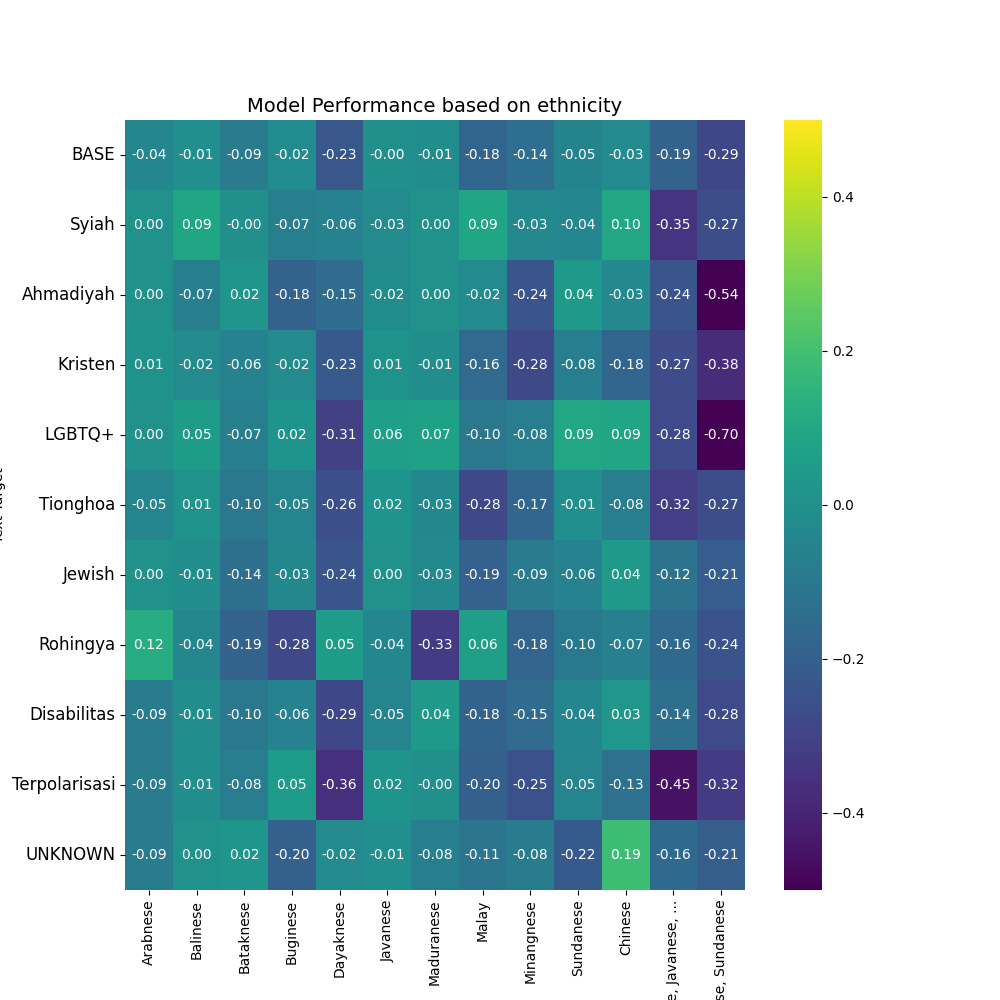}
\end{figure}
\begin{figure}
    \centering
    \includegraphics[width=1\textwidth]{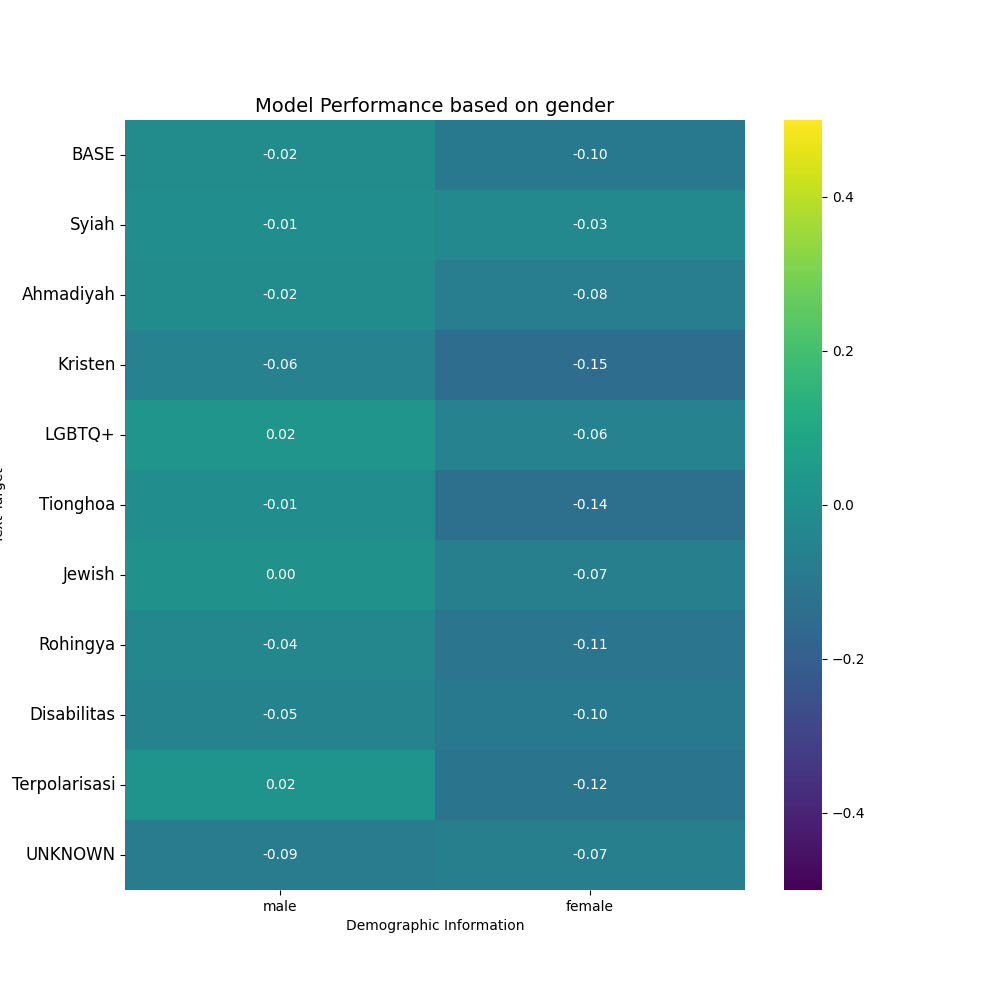}
\end{figure}
\begin{figure}
    \centering
    \includegraphics[width=1\textwidth]{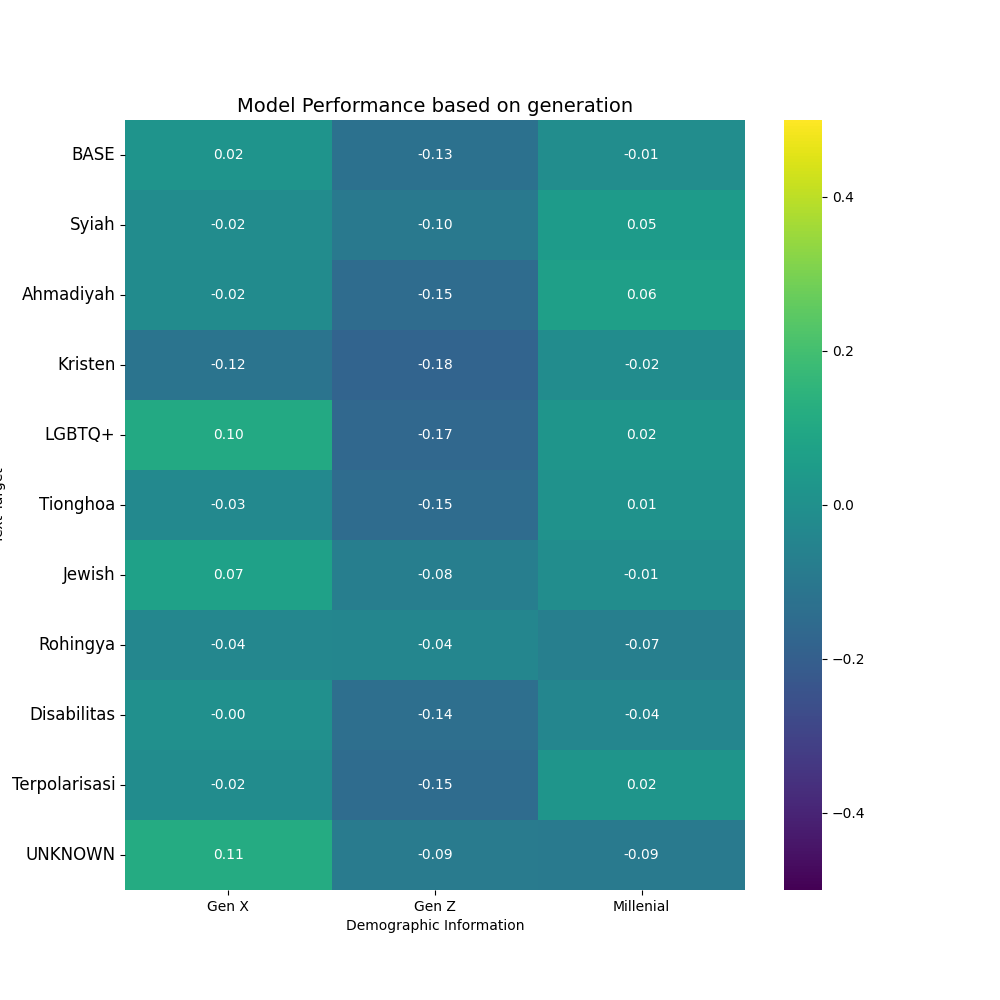}
\end{figure}
\begin{figure}
    \centering
    \includegraphics[width=1\textwidth]{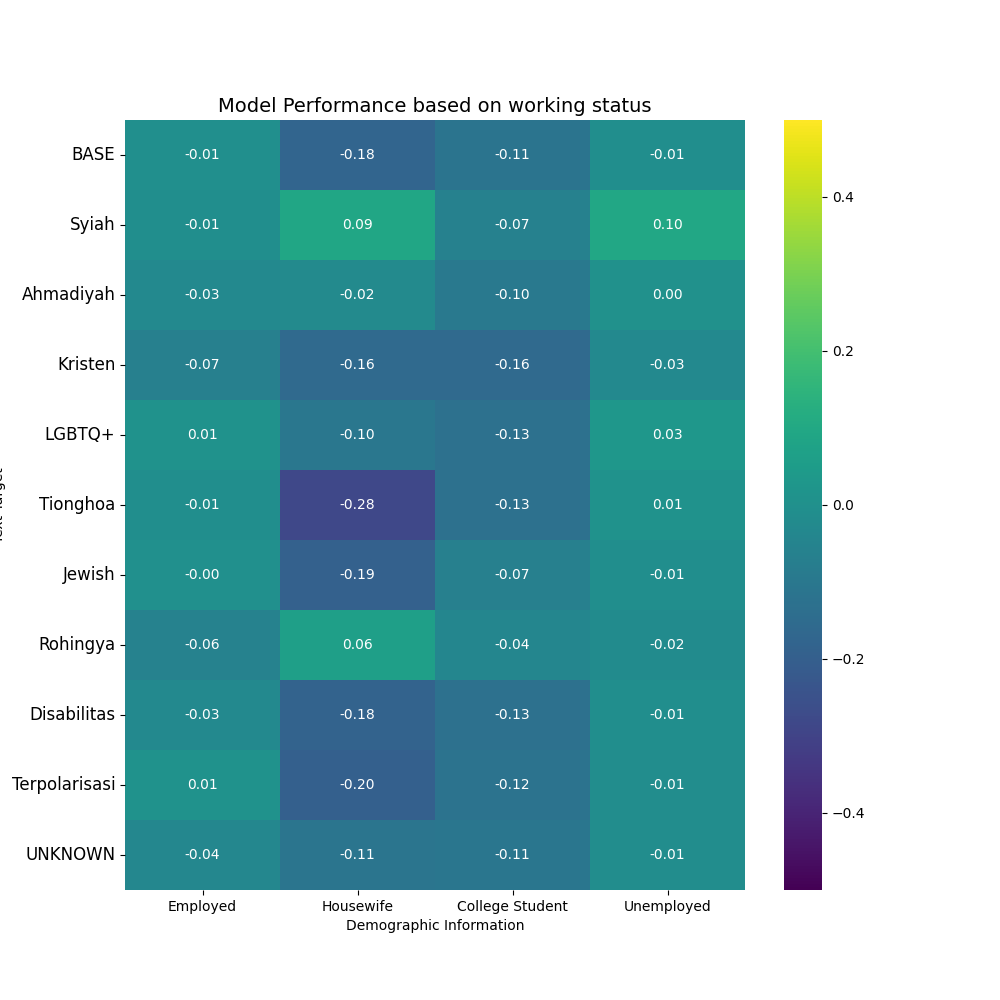}
\end{figure}
\begin{figure}
    \centering
    \includegraphics[width=1\textwidth]{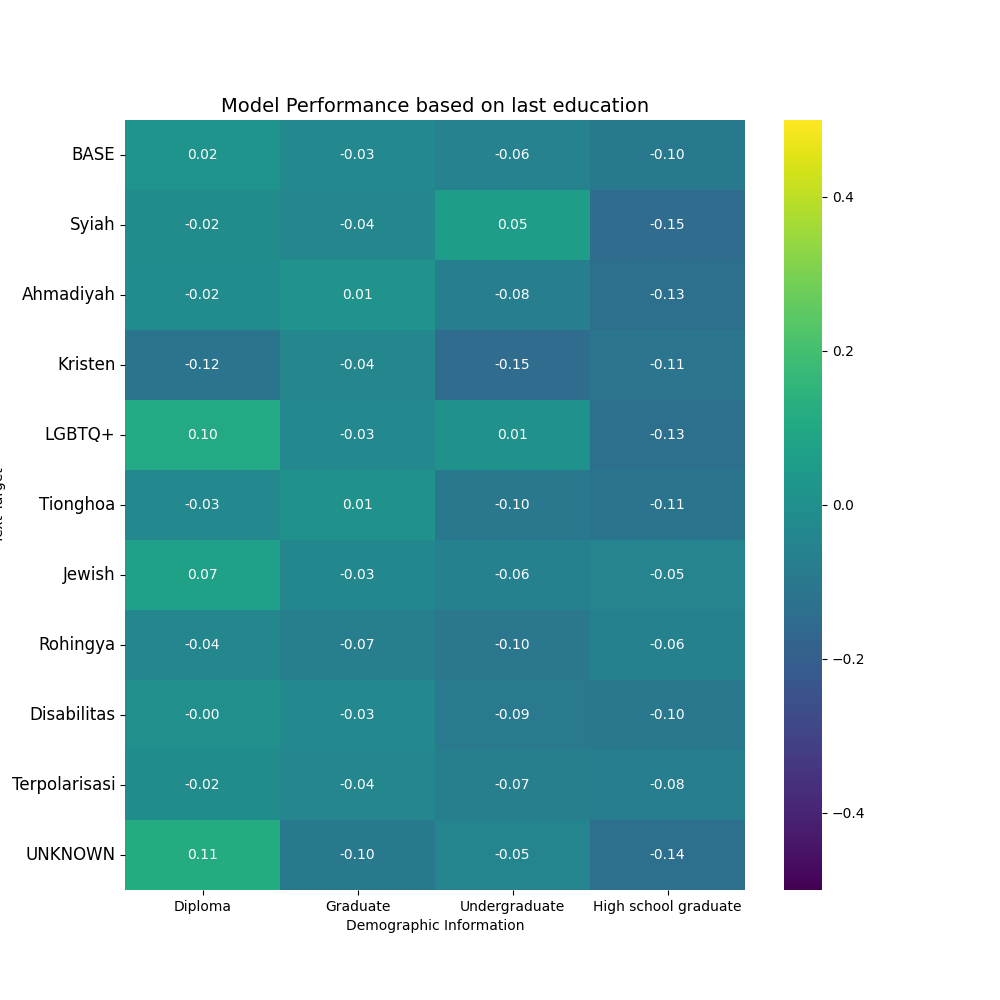}
\end{figure}
\begin{figure}
    \centering
    \includegraphics[width=1\textwidth]{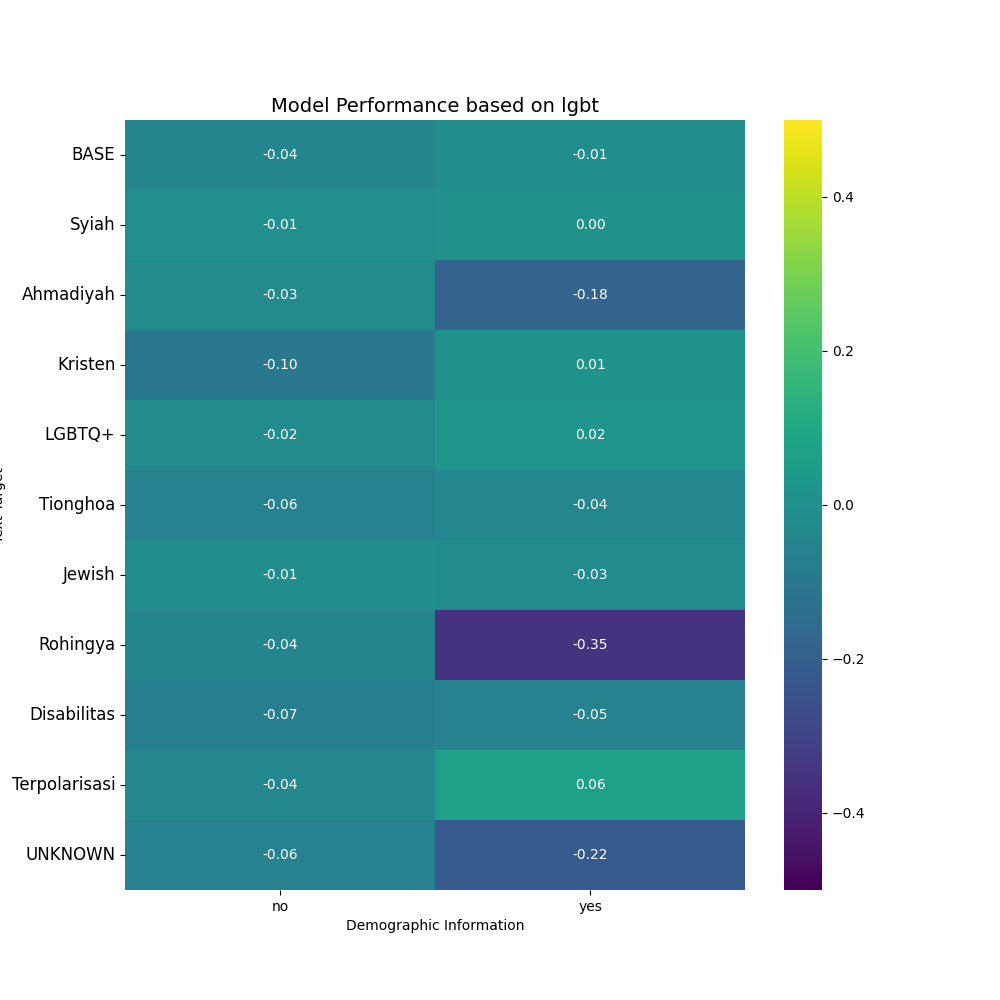}
\end{figure}
\begin{figure}
    \centering
    \includegraphics[width=1\textwidth]{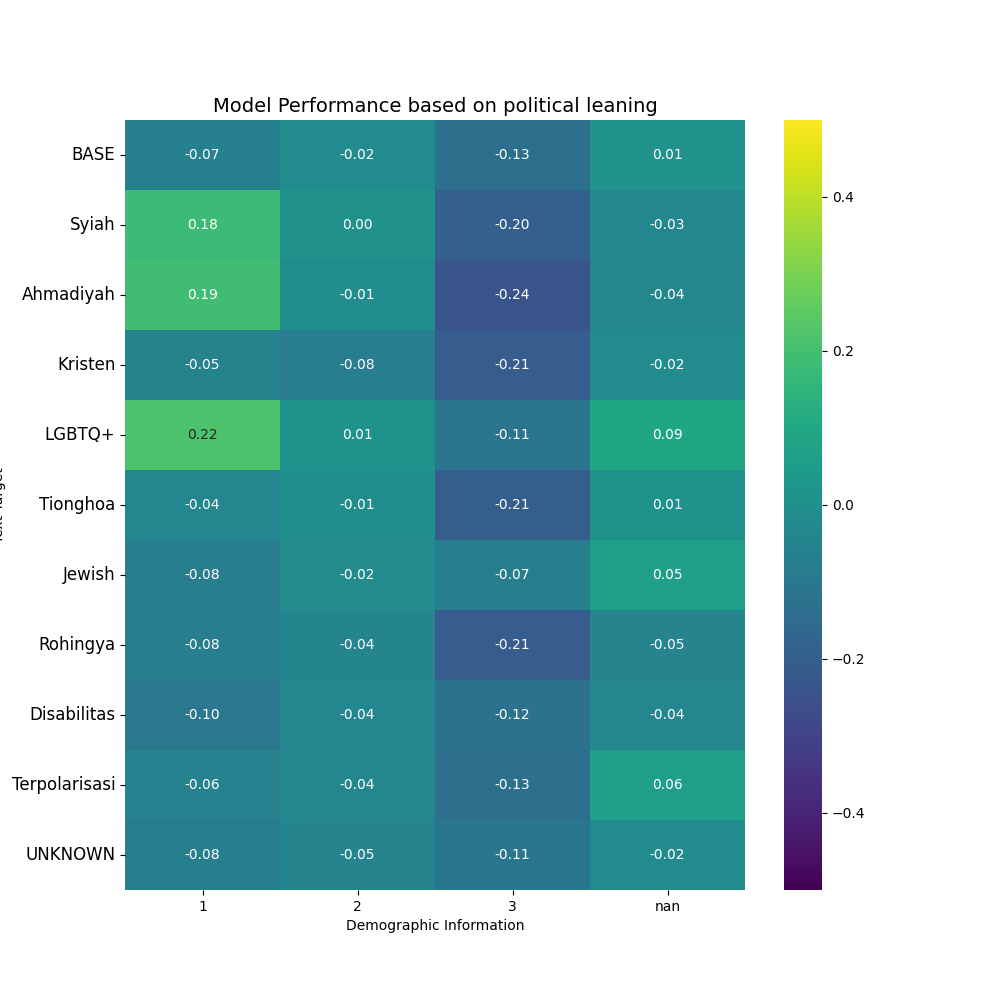}
\end{figure}
\begin{figure}
    \centering
    \includegraphics[width=1\textwidth]{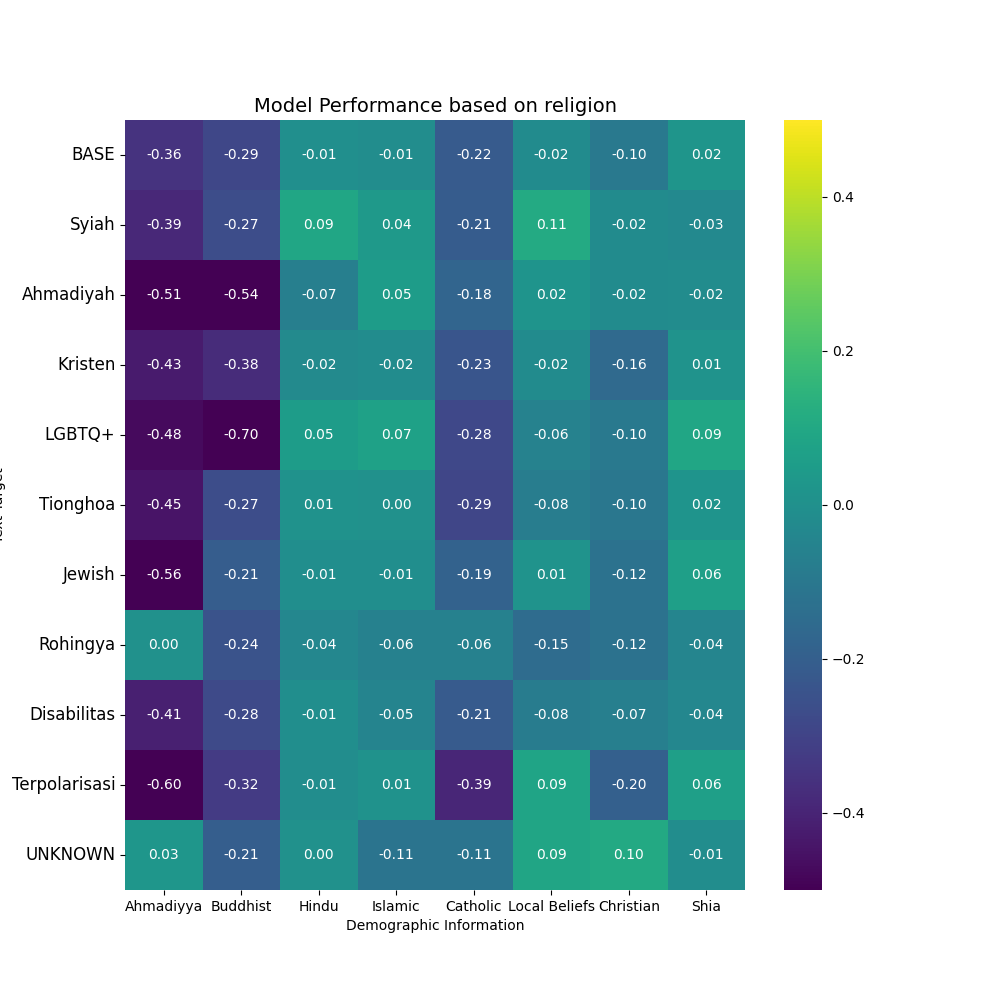}
\end{figure}

\newpage
\subsection{IndoBERTweet with Topic}
\begin{figure}[H]
    \centering
    \includegraphics[width=1\textwidth]{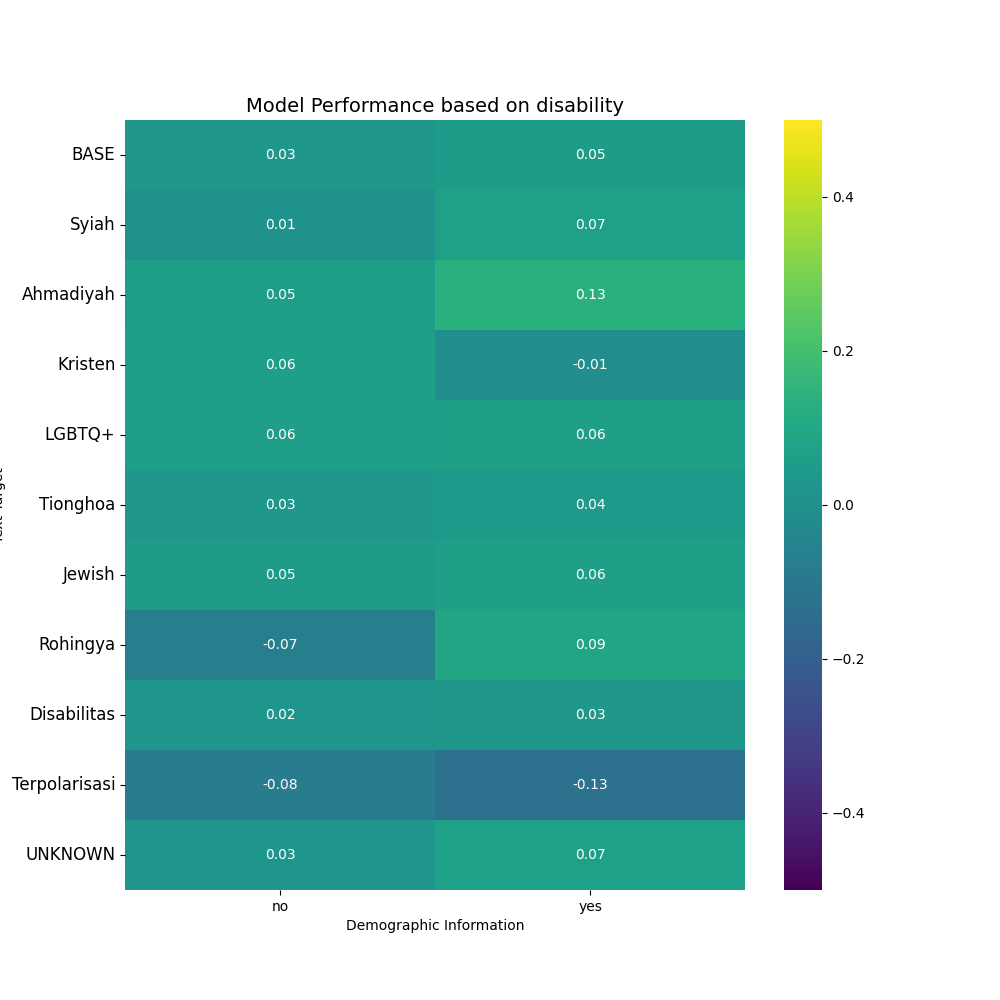}
\end{figure}
\begin{figure}
    \centering
    \includegraphics[width=1\textwidth]{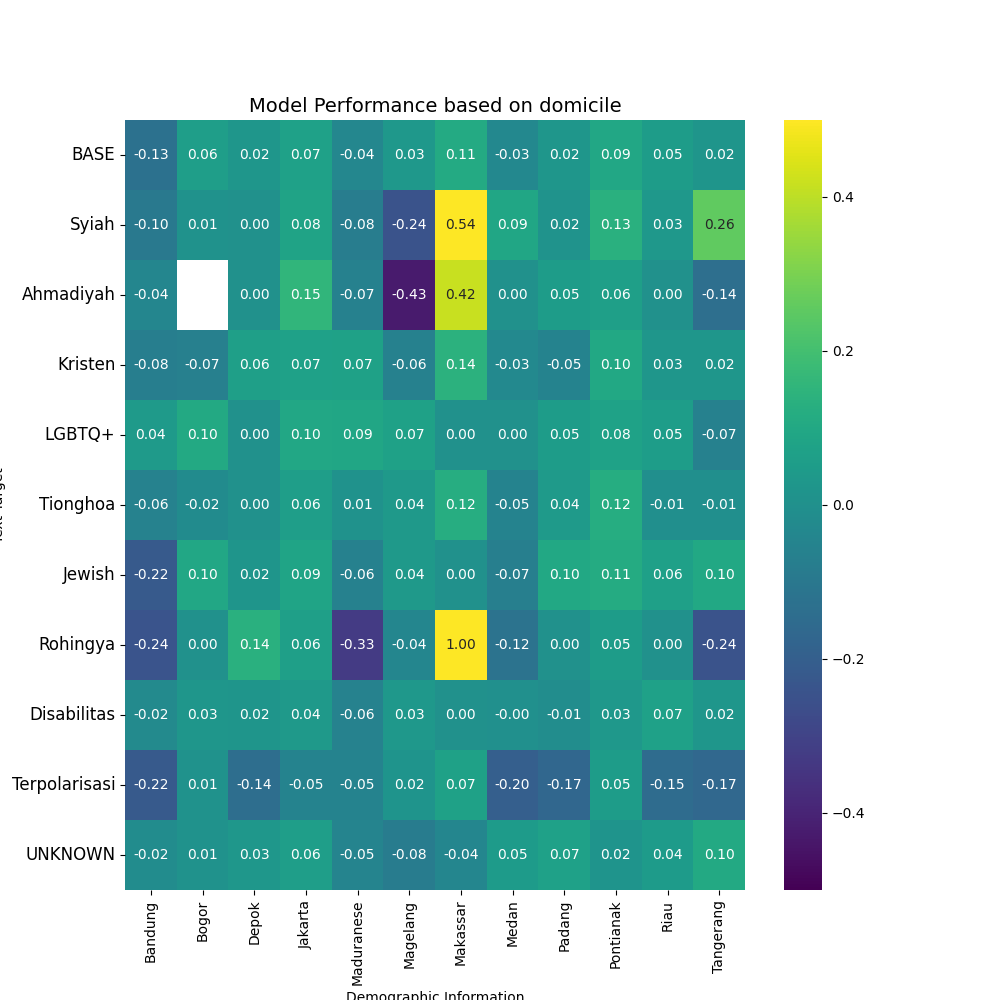}
\end{figure}
\begin{figure}
    \centering
    \includegraphics[width=1\textwidth]{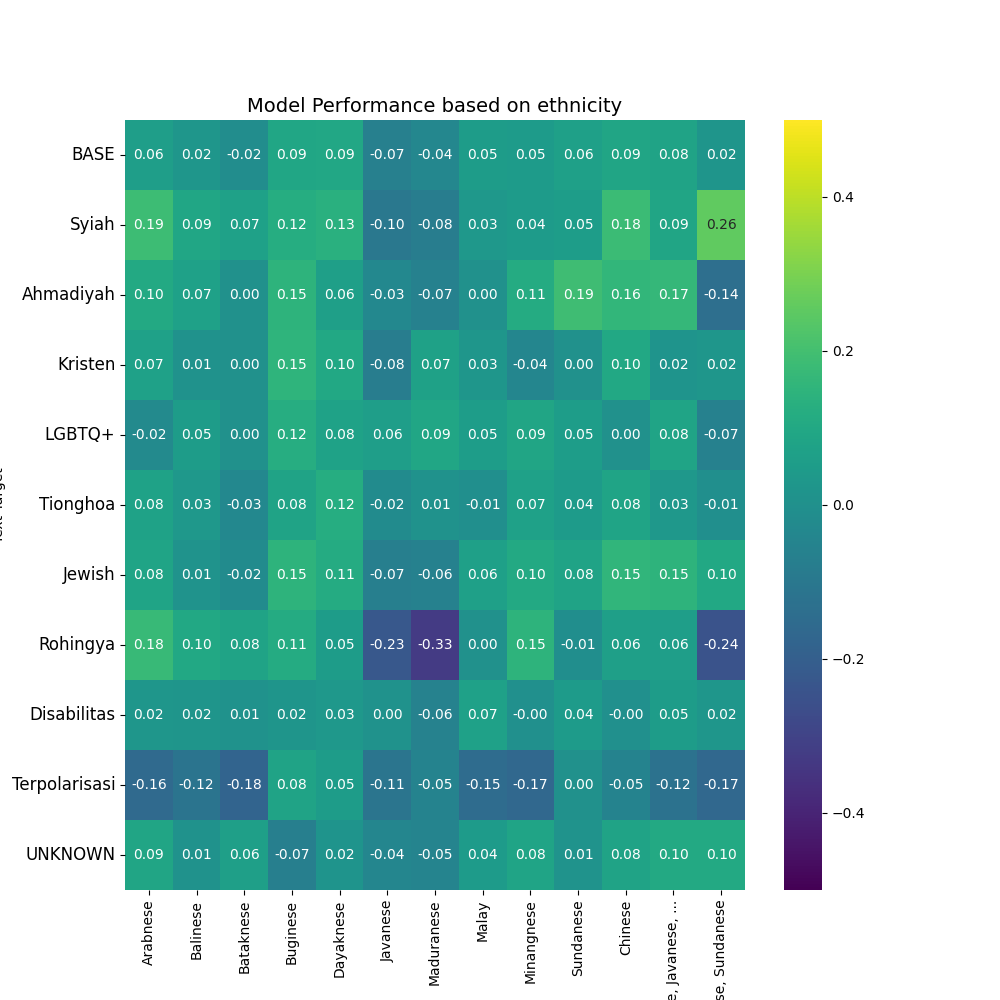}
\end{figure}
\begin{figure}
    \centering
    \includegraphics[width=1\textwidth]{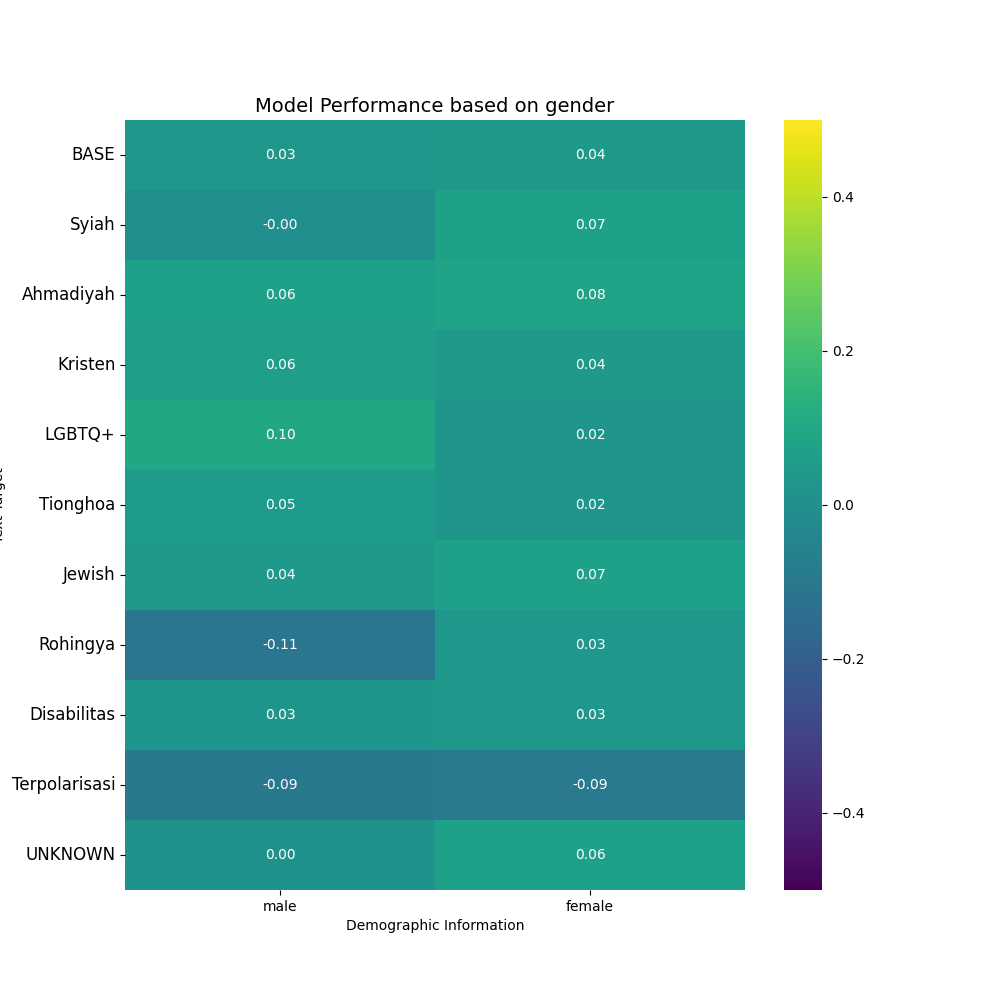}
\end{figure}
\begin{figure}
    \centering
    \includegraphics[width=1\textwidth]{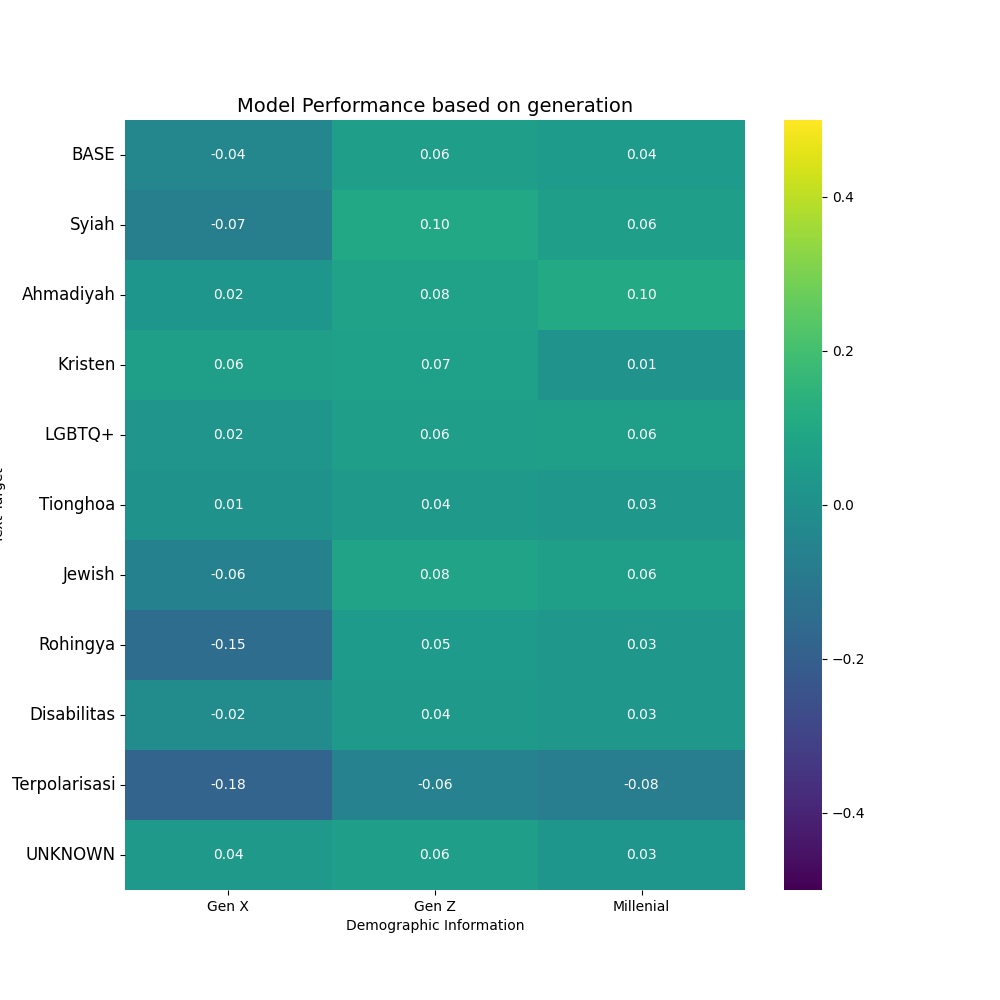}
\end{figure}
\begin{figure}
    \centering
    \includegraphics[width=1\textwidth]{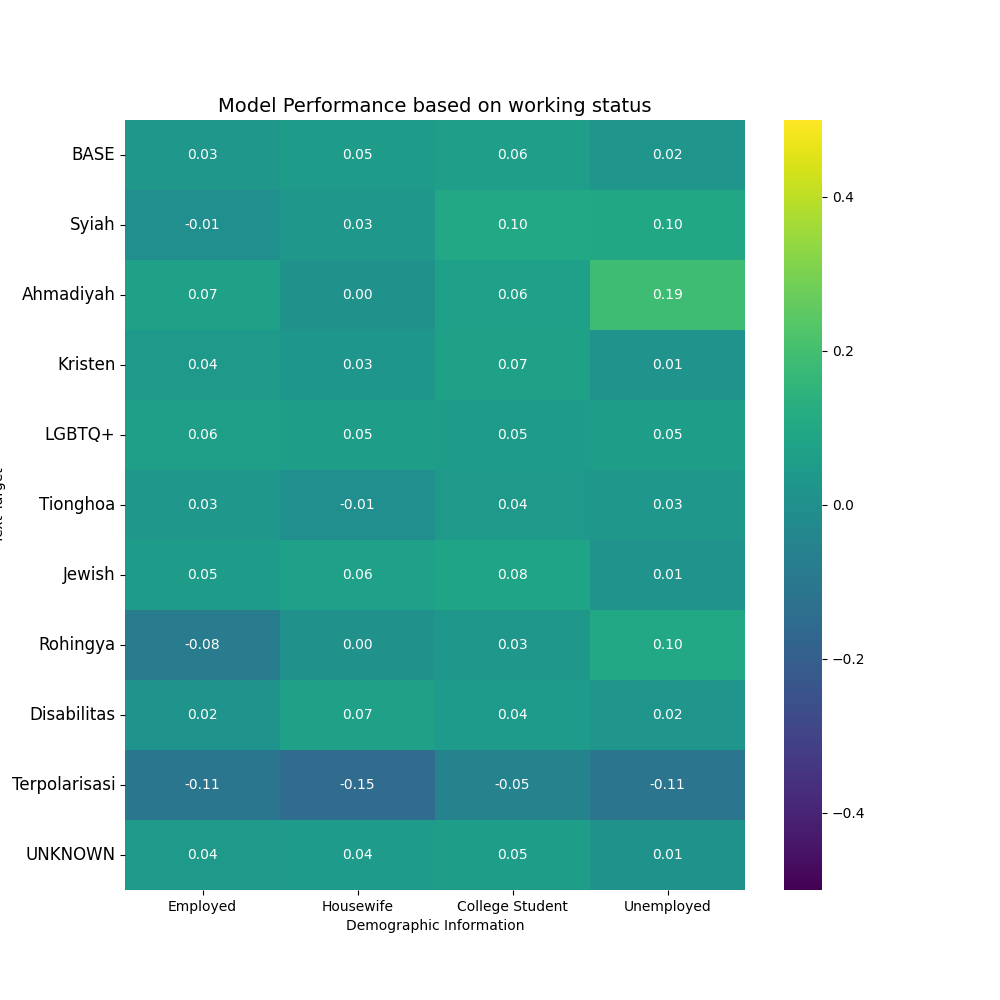}
\end{figure}
\begin{figure}
    \centering
    \includegraphics[width=1\textwidth]{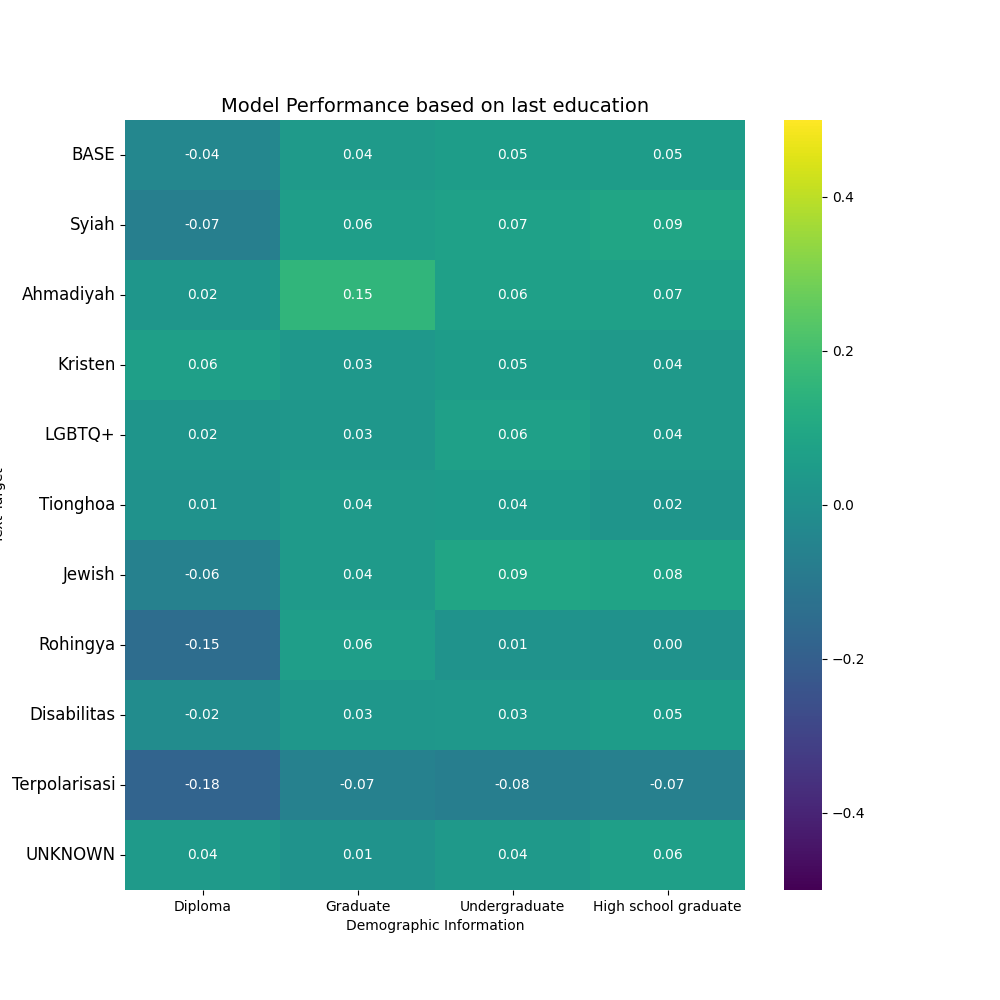}
\end{figure}
\begin{figure}
    \centering
    \includegraphics[width=1\textwidth]{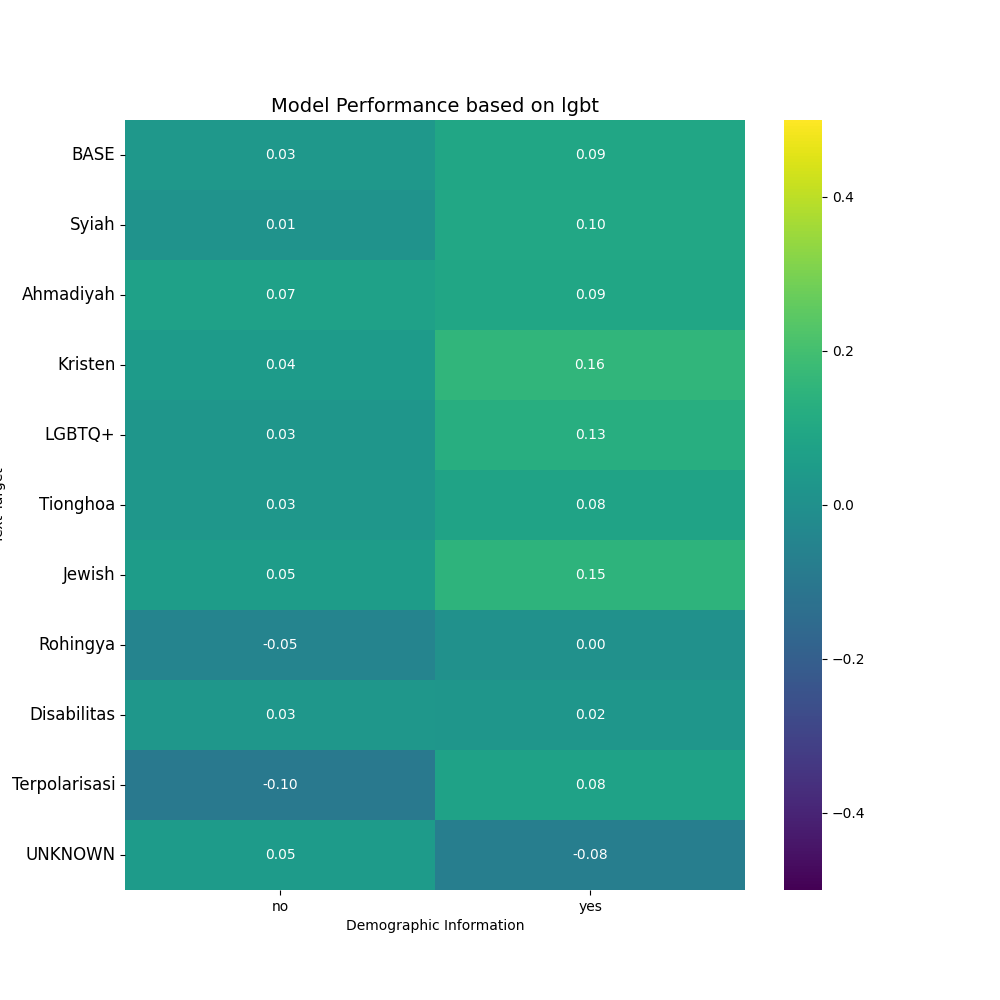}
\end{figure}
\begin{figure}
    \centering
    \includegraphics[width=1\textwidth]{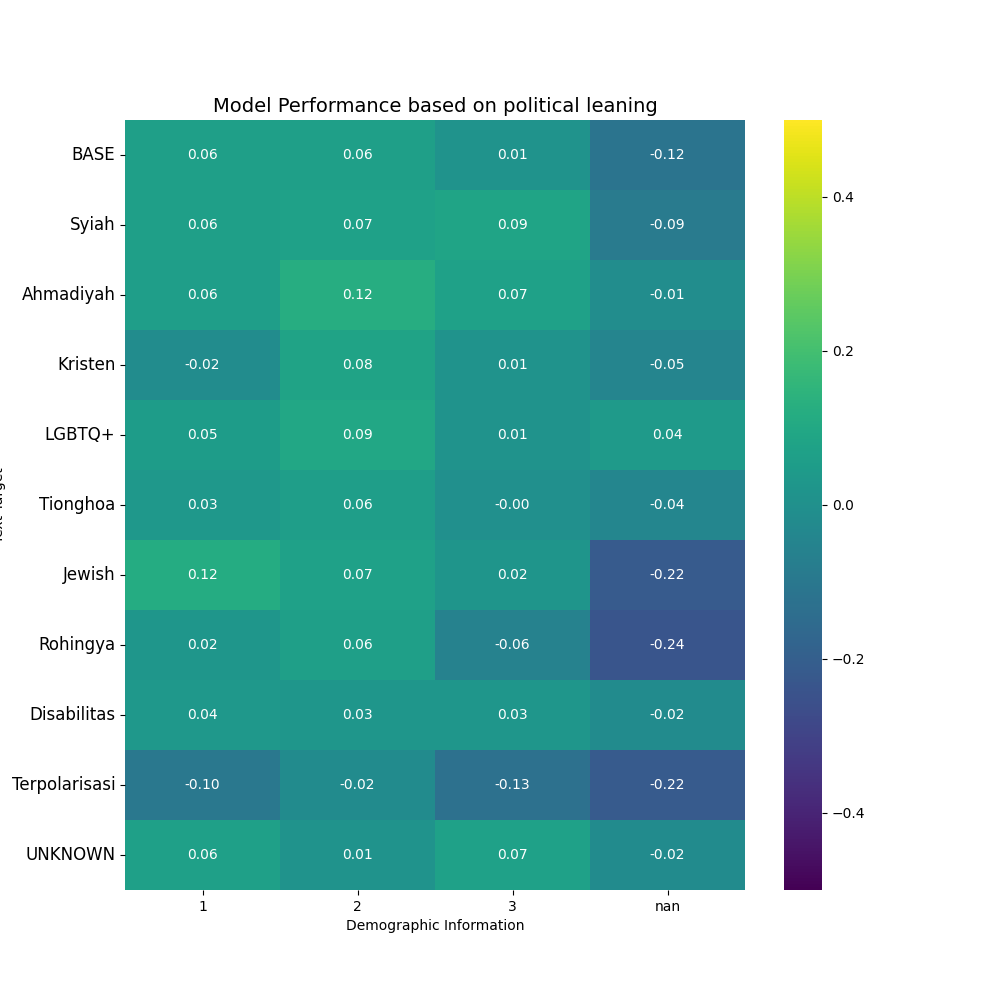}
\end{figure}
\begin{figure}
    \centering
    \includegraphics[width=1\textwidth]{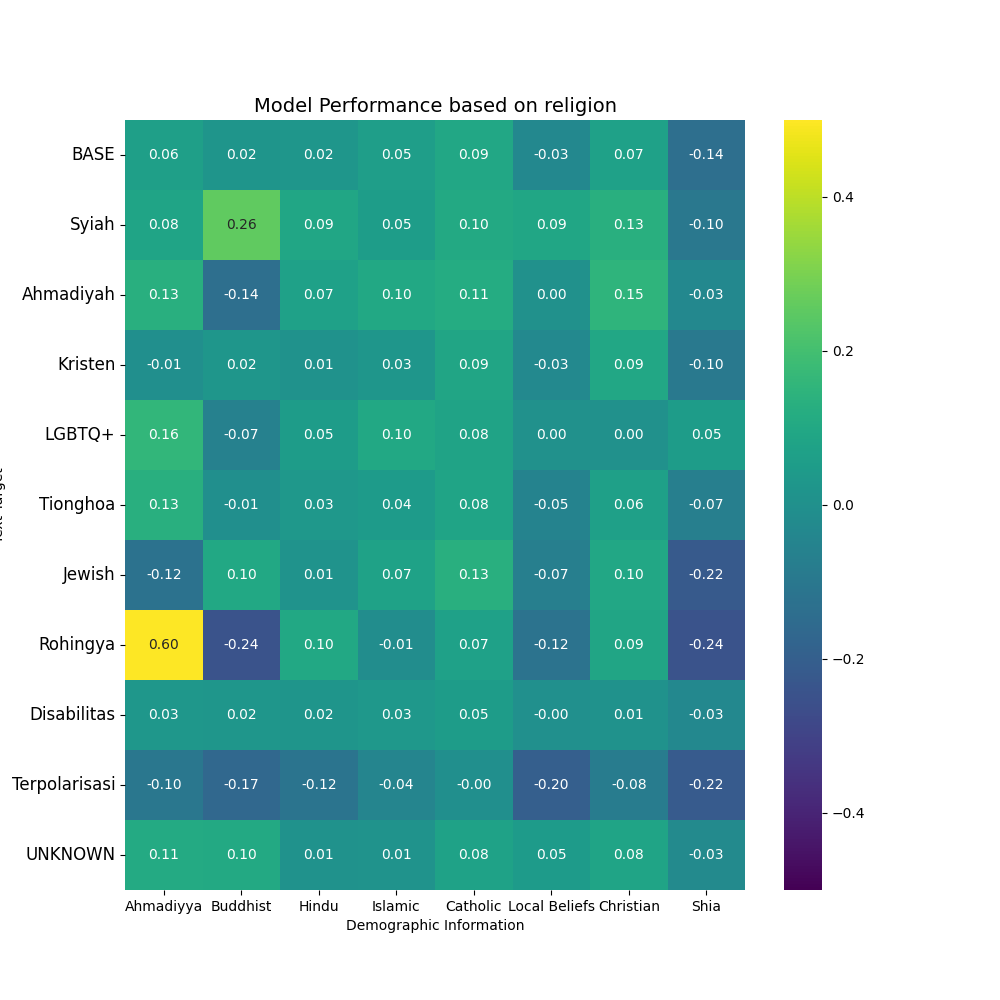}
\end{figure}

\newpage
\subsection{IndoBERTweet with Demographic and Topic}
\begin{figure}[H]
    \centering
    \includegraphics[width=1\textwidth]{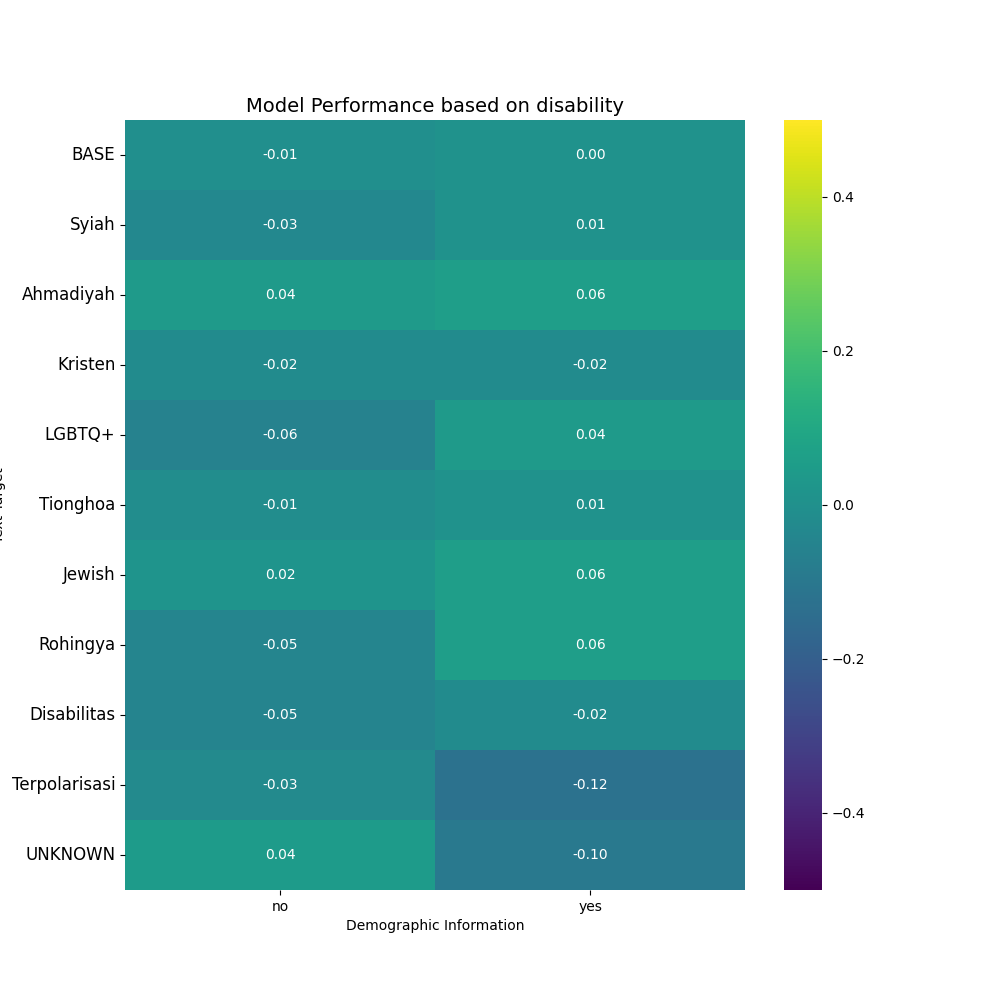}
\end{figure}
\begin{figure}
    \centering
    \includegraphics[width=1\textwidth]{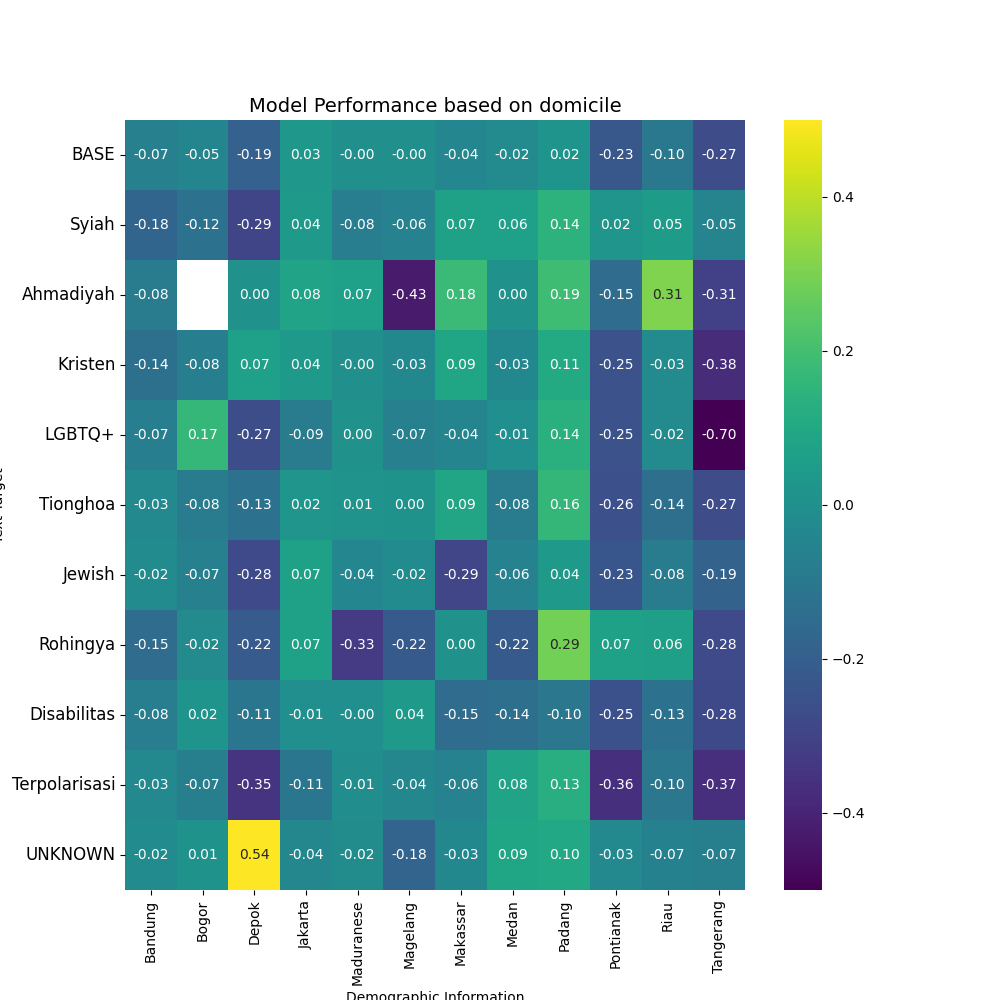}
\end{figure}
\begin{figure}
    \centering
    \includegraphics[width=1\textwidth]{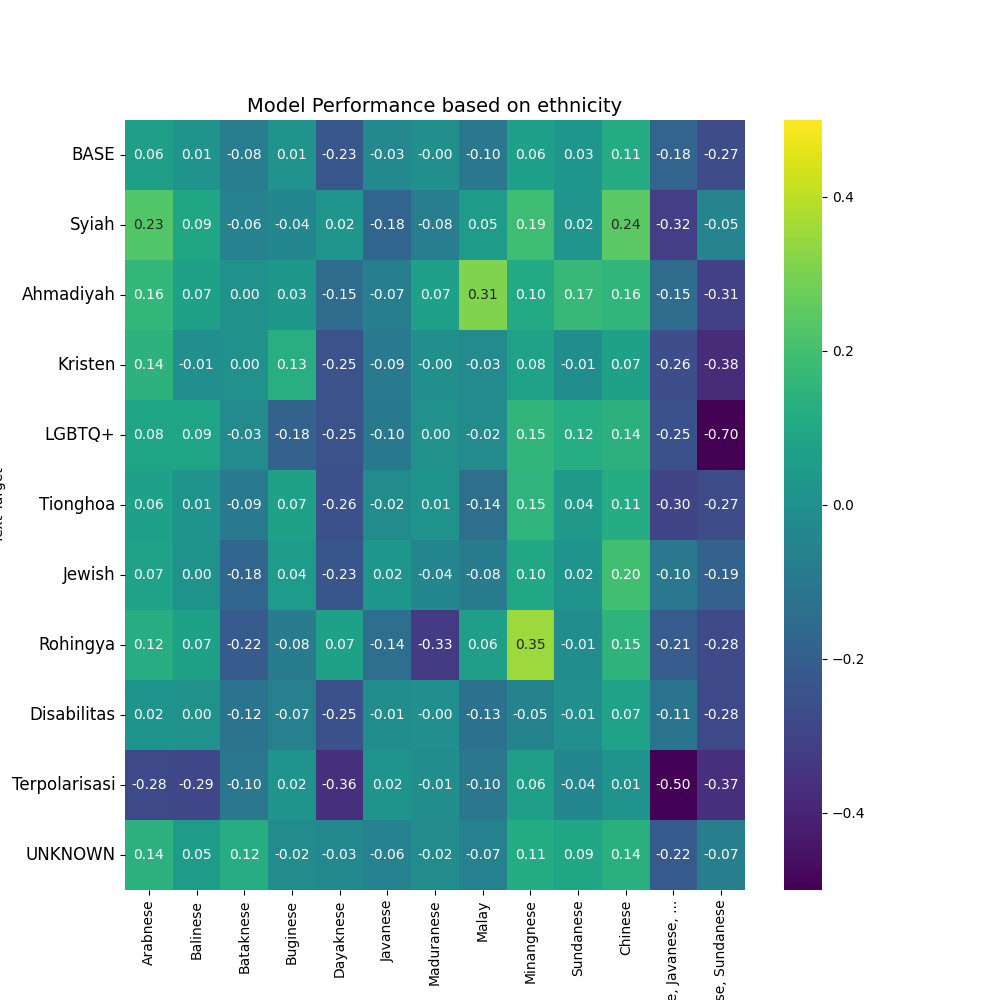}
\end{figure}
\begin{figure}
    \centering
    \includegraphics[width=1\textwidth]{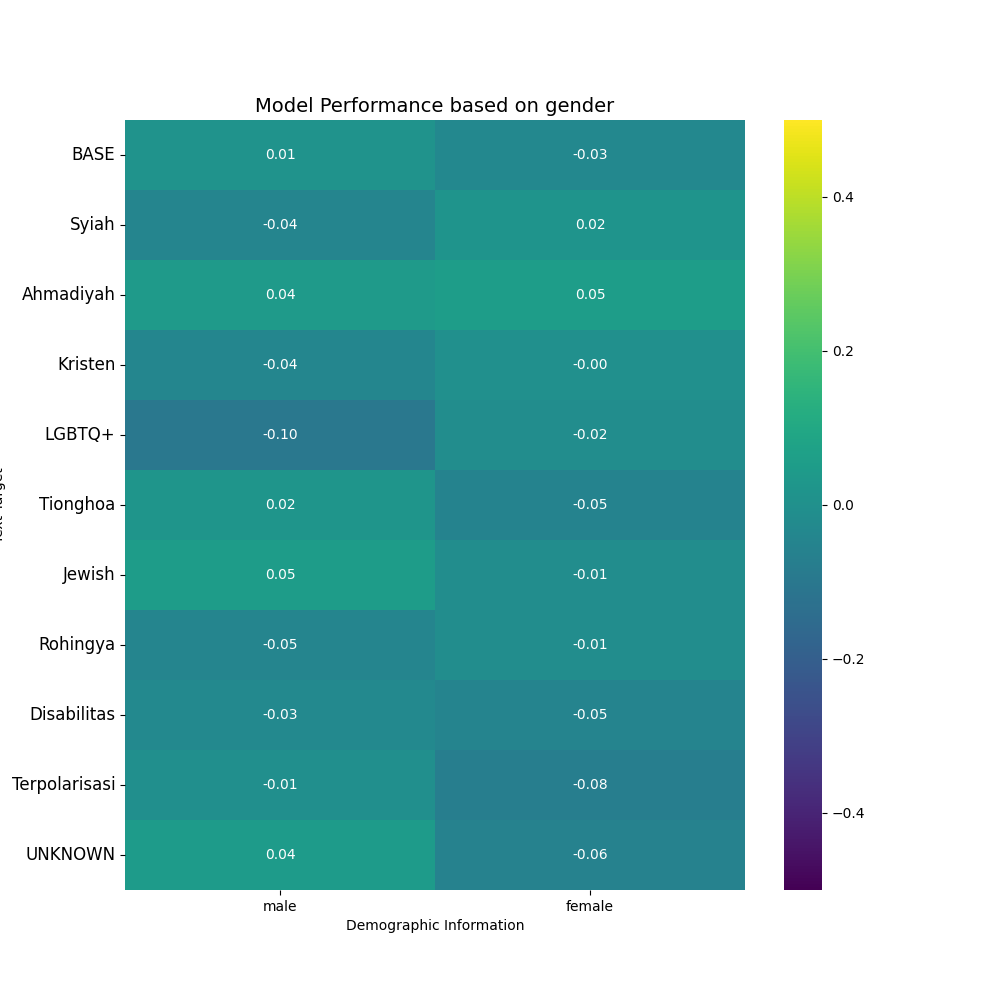}
\end{figure}
\begin{figure}
    \centering
    \includegraphics[width=1\textwidth]{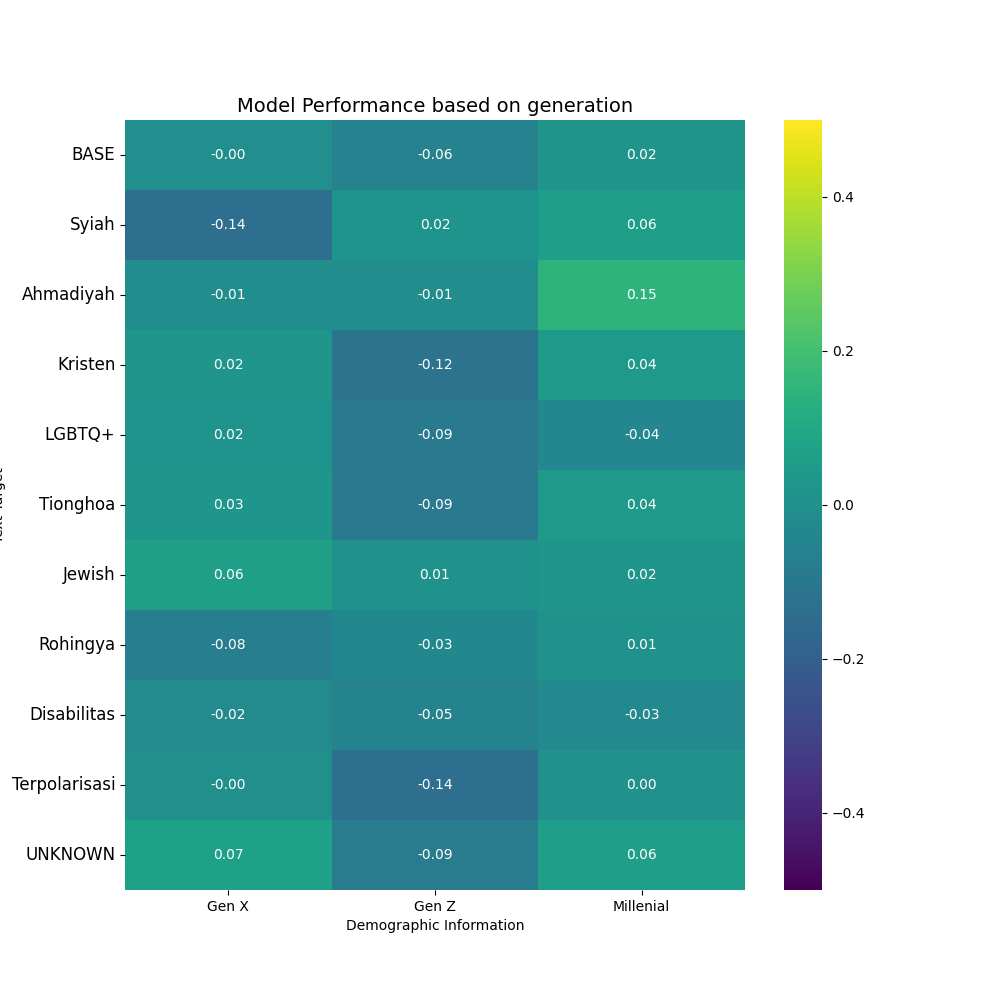}
\end{figure}
\begin{figure}
    \centering
    \includegraphics[width=1\textwidth]{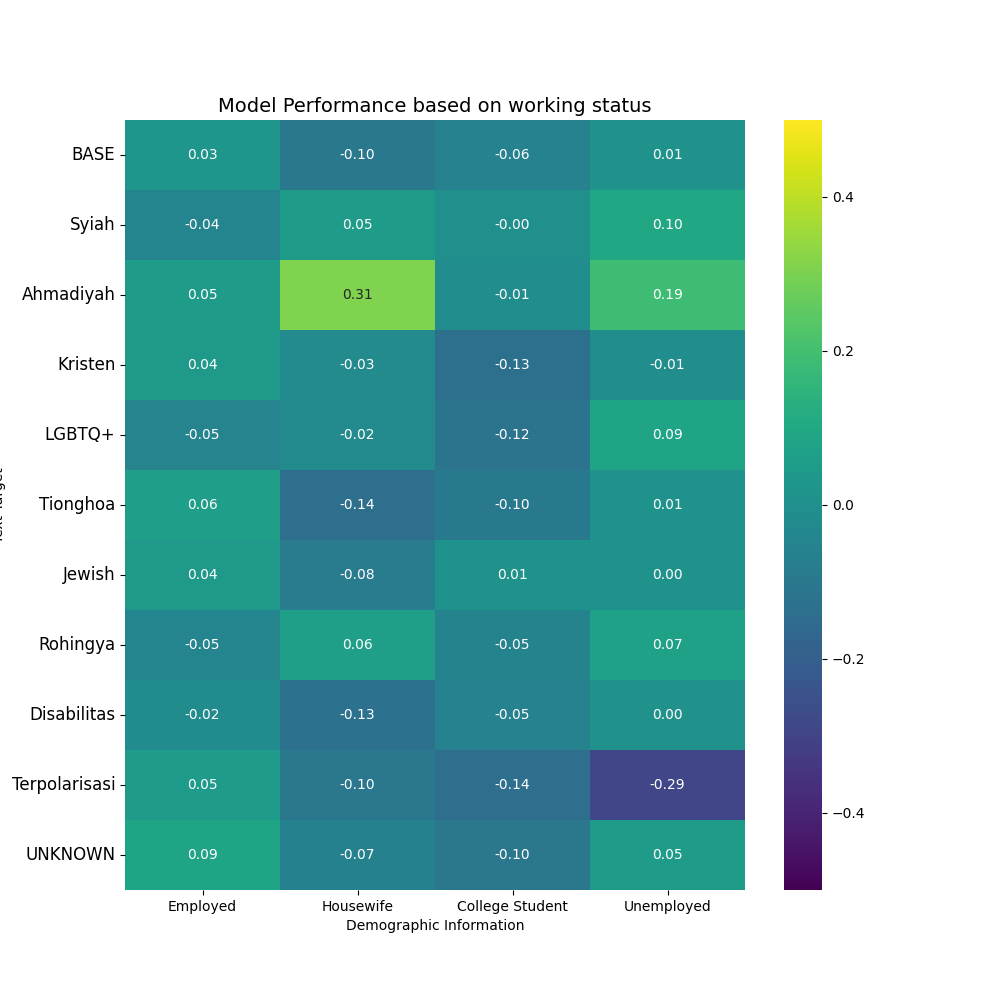}
\end{figure}
\begin{figure}
    \centering
    \includegraphics[width=1\textwidth]{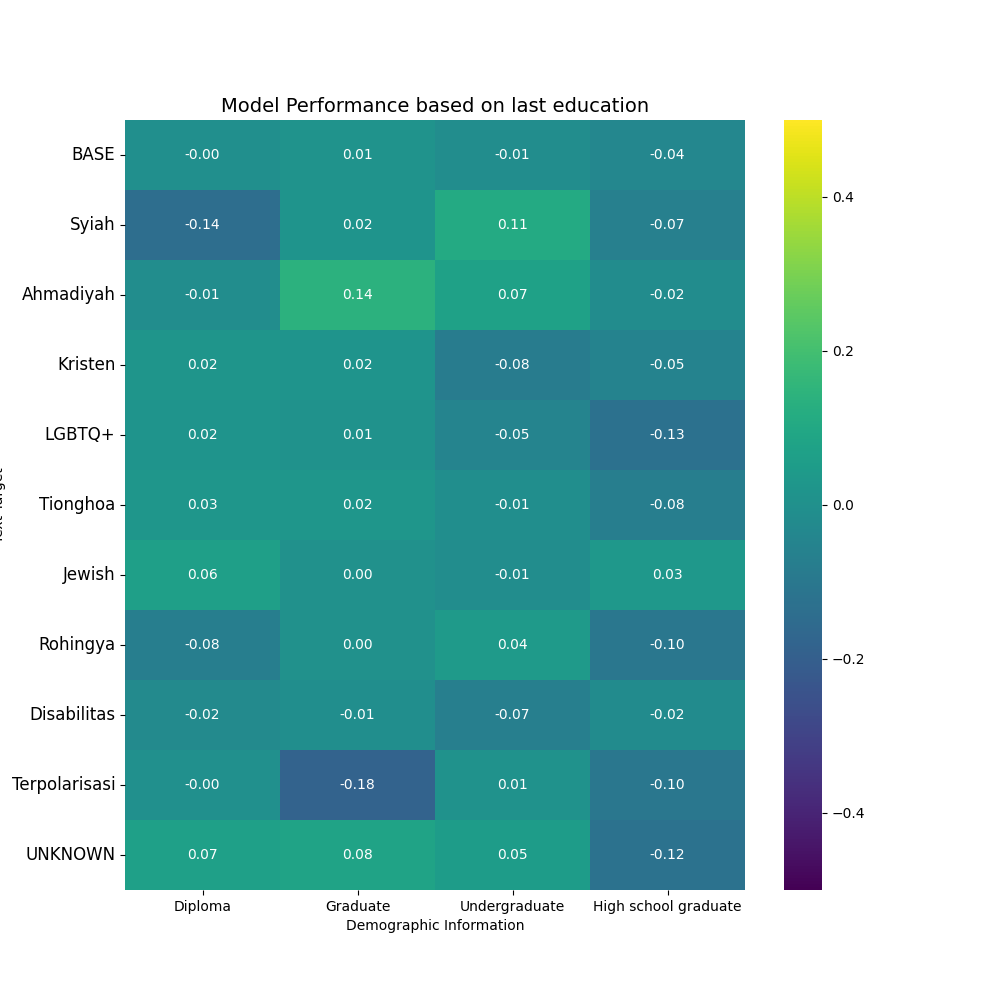}
\end{figure}
\begin{figure}
    \centering
    \includegraphics[width=1\textwidth]{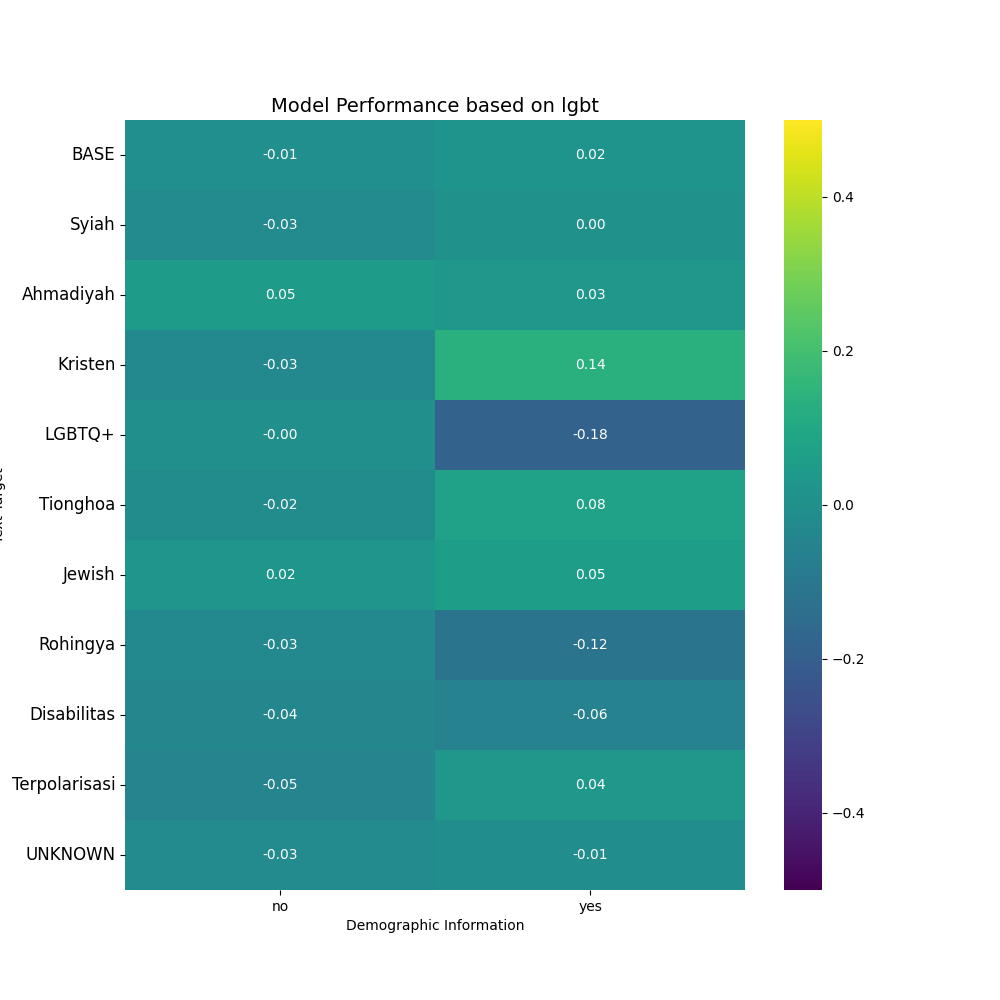}
\end{figure}
\begin{figure}
    \centering
    \includegraphics[width=1\textwidth]{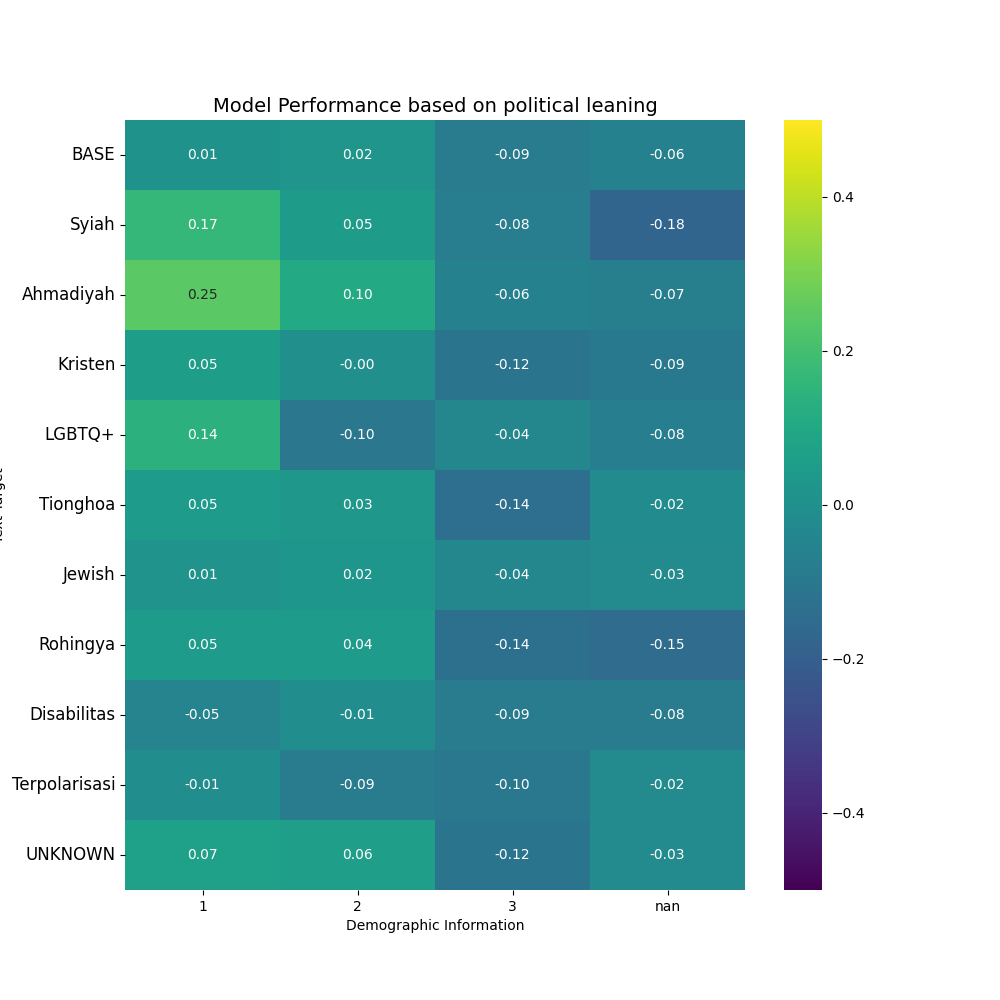}
\end{figure}
\begin{figure}
    \centering
    \includegraphics[width=1\textwidth]{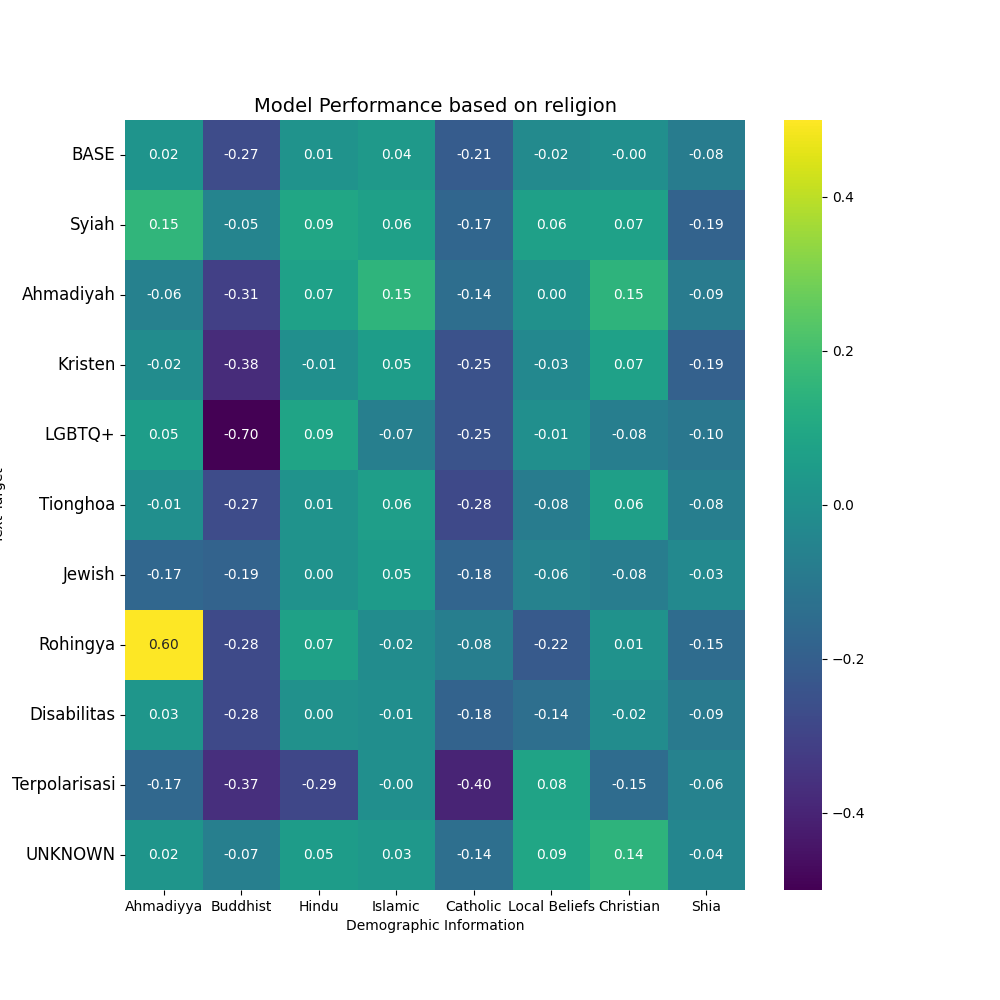}
\end{figure}
