# Supplementary material for: A Multi-Labeled Dataset for Indonesian Discourse: Examining Toxicity, Polarization, and Demographics Information
Source: arXiv:2503.00417 source file (2025-03-01)
Supplement: Supplementary file 3 [file math_notation_AC1.tex]

\section{Within \& Between Group ICR Score Calculation}
\label{sec:rigorICR}

To compute the toxicity ICR score for a demographic group, we calculate the weighted average of Gwet’s AC1 score for every pairwise combination of annotators within the same group, using the volume of text in each pair as the weight. This approach maximizes the utilization of available data. A similar calculation method is implemented to find the ICR score between two groups, with the modification that each pair consists of members from different groups. We refer to these metrics as “within-group ICR score” and “between-group ICR score” respectively.

We can rigorously define an equation to compute ICR score within a group as
\begin{equation*}
    \small
     \gamma(g)= \frac{\sum\limits_{i,j\in g}dim(v_{ij})\cdot\text{Gwet}(\phi_i(v_{ij}),\phi_j(v_{ij}))}{\sum\limits_{i,j\in g}dim(v_{ij})}
\end{equation*}

Where $g$ are an arbitrary groups in a demographic; $v_{ij}$ are set of text that both mutually by annotators $i$,$j$; and $\phi_i,\phi_j$ are annotation result from $i,j$. To calculate ICR score between two groups, we slightly modified the equation above into

\begin{equation*}
    \small
     \Gamma(g_1,g_2)= \frac{\sum\limits_{i\in g_1,j \in g_2}dim(v_{ij})\cdot\text{Gwet}(\phi_i(v_{ij}),\phi_j(v_{ij}))}{\sum\limits_{i\in g_1,j \in g_2}dim(v_{ij})}
\end{equation*}

Where $g_1$,$g_2$ are arbitrary two groups in a demographic; $v_{ij}$ are set of text that both mutually by annotators $i$,$j$; and $\phi_i,\phi_j$ are annotation result from $i,j$.
