# Supplementary material for: A Multi-Labeled Dataset for Indonesian Discourse: Examining Toxicity, Polarization, and Demographics Information
Source: arXiv:2503.00417 source file (2025-03-01)
Supplement: Supplementary file 4 [file train_test_different_demography.tex]

\section{Model Performance When Trained and Tested on Different Demographic Groups}
\label{app:model-cross-demographics}
\noindent
\begin{minipage}{0.58\textwidth}
    \centering
    \begin{tabular*}{\textwidth}{@{\extracolsep{\fill}}*{3}{c}}
        \toprule
        \multicolumn{1}{l}{\textbf{Train on}} & 
        \multicolumn{2}{c}{\textbf{Test on}}\\
        \cline{2-3} 
         & No Disability & With Disability \\
        \midrule
        \multicolumn{1}{>{\hspace{0pt}}m{0.25\linewidth}}{No Disability} & 0.642 & 0.635  \\
        \multicolumn{1}{>{\hspace{0pt}}m{0.25\linewidth}}{With Disability}     & 0.602 & 0.627  \\
        \bottomrule
    \end{tabular*}
    \captionof{table}{Disability demographic groups.}
\end{minipage}%
\hspace{15pt}
\begin{minipage}{0.42\textwidth}
    \centering
    \begin{tabular*}{\textwidth}{@{\extracolsep{\fill}}*{3}{c}}
        \toprule
        \multicolumn{1}{l}{\textbf{Train on}} & 
        \multicolumn{2}{c}{\textbf{Test on}}\\
        \cline{2-3} 
         & Female & Male \\
        \midrule
        \multicolumn{1}{>{\hspace{0pt}}m{0.25\linewidth}}{Female} & 0.511 & 0.587  \\
        \multicolumn{1}{>{\hspace{0pt}}m{0.25\linewidth}}{Male}  & 0.548 & 0.673  \\
        \bottomrule
    \end{tabular*}
    \captionof{table}{Gender demographic groups.}
\end{minipage} \vspace{25pt}\\

\noindent
\begin{minipage}{0.9\textwidth}
    \begin{center}
         \begin{tabular*}{\textwidth}{@{\extracolsep{\fill}}*{4}{c}}
            \toprule
            \multicolumn{1}{l}{\textbf{Train on}} & 
            \multicolumn{3}{c}{\textbf{Test on}}\\
            \cline{2-4} 
             & Bachelor's Degree & High school Degree & Master's Degree \\
            \midrule
            \multicolumn{1}{>{\hspace{0pt}}m{0.25\linewidth}}{Bachelor's Degree} & 0.562 & 0.354 & 0.619 \\
            \multicolumn{1}{>{\hspace{0pt}}m{0.25\linewidth}}{High school Degree}  & 0.267 & 0.236 & 0.284 \\
            \multicolumn{1}{>{\hspace{0pt}}m{0.25\linewidth}}{Master's Degree}  & 0.590 & 0.347 & 0.746 \\
            \bottomrule
        \end{tabular*}
        \captionof{table}{Education demographic groups.}
    \end{center}
\end{minipage}\vspace{25pt}\\

\noindent
\begin{minipage}{0.57\textwidth}
    \begin{center}
         \begin{tabular*}{\textwidth}{lccc}
            \toprule
            \textbf{Train on} & 
            \multicolumn{3}{c}{\textbf{Test on}}\\
            \cline{2-4} 
             & Employed & In College & Unemployed \\
            \midrule
            \multicolumn{1}{>{\hspace{0pt}}m{0.25\linewidth}}{Employed} & 0.653 & 0.389 & 0.644 \\
            \multicolumn{1}{>{\hspace{0pt}}m{0.25\linewidth}}{In College}  & 0.446 & 0.288 & 0.418 \\
            \multicolumn{1}{>{\hspace{0pt}}m{0.25\linewidth}}{Unemployed}  & 0.650 & 0.368 & 0.649 \\
            \bottomrule
        \end{tabular*}
        \captionof{table}{Job status demographic groups.}
    \end{center}
\end{minipage}
\hspace{15pt}
\begin{minipage}{0.44\textwidth}
    \begin{center}
         \begin{tabular*}{\textwidth}{lccc}
            \toprule
            \textbf{Train on}& 
            \multicolumn{3}{c}{\textbf{Test on}}\\
            \cline{2-4} 
             & Gen X & Gen Z & Millennial \\
            \midrule
            \multicolumn{1}{>{\hspace{0pt}}m{0.25\linewidth}}{Gen X} & 0.496 & 0.288 & 0.385 \\
            \multicolumn{1}{>{\hspace{0pt}}m{0.25\linewidth}}{Gen Z}  & 0.447 & 0.431 & 0.508 \\
            \multicolumn{1}{>{\hspace{0pt}}m{0.25\linewidth}}{Millennial}  & 0.545 & 0.451 & 0.687 \\
            \bottomrule
        \end{tabular*}
        \captionof{table}{Age demographic groups.}
    \end{center}
\end{minipage}\vspace{25pt}\\

\noindent
\begin{minipage}{0.5\textwidth}
    \begin{center}
         \begin{tabular*}{\textwidth}{lcc}
            \toprule
            \textbf{Train on} & 
            \multicolumn{2}{c}{\textbf{Test on}}\\
            \cline{2-3} 
              &Live in Java&Live outside Java\\
            \midrule
            \multicolumn{1}{>{\hspace{0pt}}m{0.25\linewidth}}{in Java} & 0.671 & 0.510  \\
            \multicolumn{1}{>{\hspace{0pt}}m{0.25\linewidth}}{outside Java}  & 0.488 & 0.481  \\
            \bottomrule
        \end{tabular*}
        \captionof{table}{Domicile (living in java island or outside java) demographic.}
    \end{center}
\end{minipage}
\hspace{15pt}
\begin{minipage}{0.5\textwidth}
    \begin{center}
         \begin{tabular*}{\textwidth}{@{\extracolsep{\fill}}*{3}{c}}
            \toprule
            \multicolumn{1}{l}{\textbf{Train on}} & 
            \multicolumn{2}{c}{\textbf{Test on}}\\
            \cline{2-3} 
              &Chinese&non-Chinese\\
            \midrule
            \multicolumn{1}{>{\hspace{0pt}}m{0.25\linewidth}}{Chinese} & 0.401& 0.342  \\
            \multicolumn{1}{>{\hspace{0pt}}m{0.25\linewidth}}{non-Chinese}  & 0.451 & 0.660  \\
            \bottomrule
        \end{tabular*}
        \captionof{table}{Ethnicity (Chinese descendant vs non-Chinese descendant) demographic.}
    \end{center}
\end{minipage}\vspace{25pt}\\

\noindent
\begin{minipage}{0.52\textwidth}
    \begin{center}
         \begin{tabular*}{\textwidth}{lcc}
            \toprule
            \textbf{Train on} & 
            \multicolumn{2}{c}{\textbf{Test on}}\\
            \cline{2-3} 
              &Ethnic in Java&Ethnic outside Java\\
            \midrule
            \multicolumn{1}{>{\hspace{0pt}}m{0.25\linewidth}}{in Java} & 0.628 & 0.572  \\
            \multicolumn{1}{>{\hspace{0pt}}m{0.25\linewidth}}{outside Java}  & 0.590 & 0.595  \\
            \bottomrule
        \end{tabular*}
        \captionof{table}{Ethnicity groups with origin from java (Javanese, Sundanese, etc) versus ethnicity from outside Java, such as
        Batak, Dayak, etc.}
    \end{center}
\end{minipage}
\hspace{15pt}
\begin{minipage}{0.49\textwidth}
    \begin{center}
         \begin{tabular*}{\textwidth}{@{\extracolsep{\fill}}*{4}{c}}
            \toprule
            \multicolumn{1}{l}{\textbf{Train on}} & 
            \multicolumn{3}{c}{\textbf{Test on}}\\
            \cline{2-4} 
              &1& 2& 3\\
            \midrule
            \multicolumn{1}{>{\hspace{0pt}}m{0.25\linewidth}}{1} & 0.440 & 0.510 & 0.351 \\
            \multicolumn{1}{>{\hspace{0pt}}m{0.25\linewidth}}{2} & 0.491 & 0.693 & 0.447 \\
            \multicolumn{1}{>{\hspace{0pt}}m{0.25\linewidth}}{3}  & 0.342 & 0.441 & 0.388\\
            \bottomrule
        \end{tabular*}
        \captionof{table}{Presidential vote candidate (Candidate 1: Anies, Candidate 2: Prabowo, or Candidate 3: Ganjar) demographic groups.}
    \end{center}
\end{minipage}\vspace{25pt}\\
