# Supplementary material for: A Multi-Labeled Dataset for Indonesian Discourse: Examining Toxicity, Polarization, and Demographics Information
Source: arXiv:2503.00417 source file (2025-03-01)
Supplement: Supplementary file 5 [file demotopic_f1.tex]

\section{Performance of Fine-tuned Models on Multiple Topics}
\label{app:f1_demotopic}

The figures below show the performance of our fine-tuned models, trained per demographic group, on various text topics. As the demographic group changes, the performance of each model also differs per topic.

\begin{figure}[h]
    \centering
    \includegraphics[width=1\textwidth]{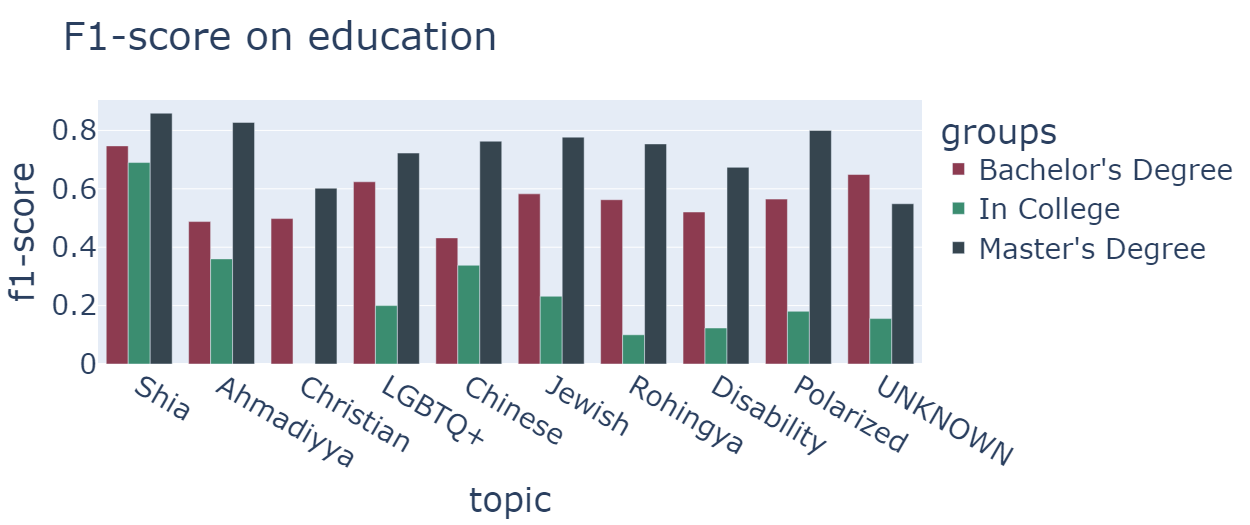}
    \label{fig:demotopic-education}
\end{figure}
\begin{figure}[h]
    \centering
    \includegraphics[width=1\textwidth]{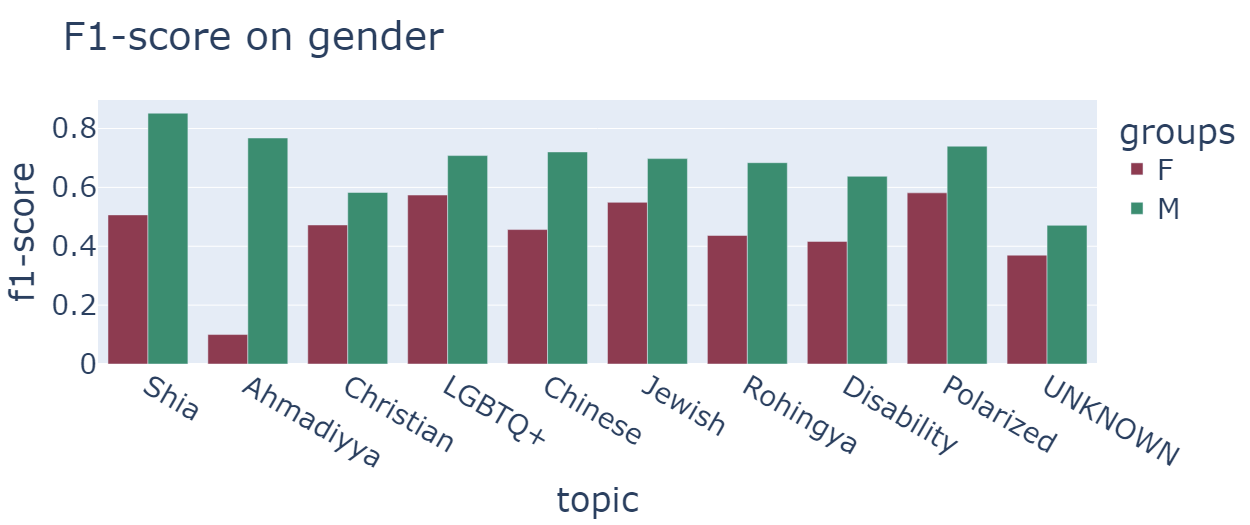}
    \label{fig:demotopic-gender}
\end{figure}
\begin{figure}[h]
    \centering
    \includegraphics[width=1\textwidth]{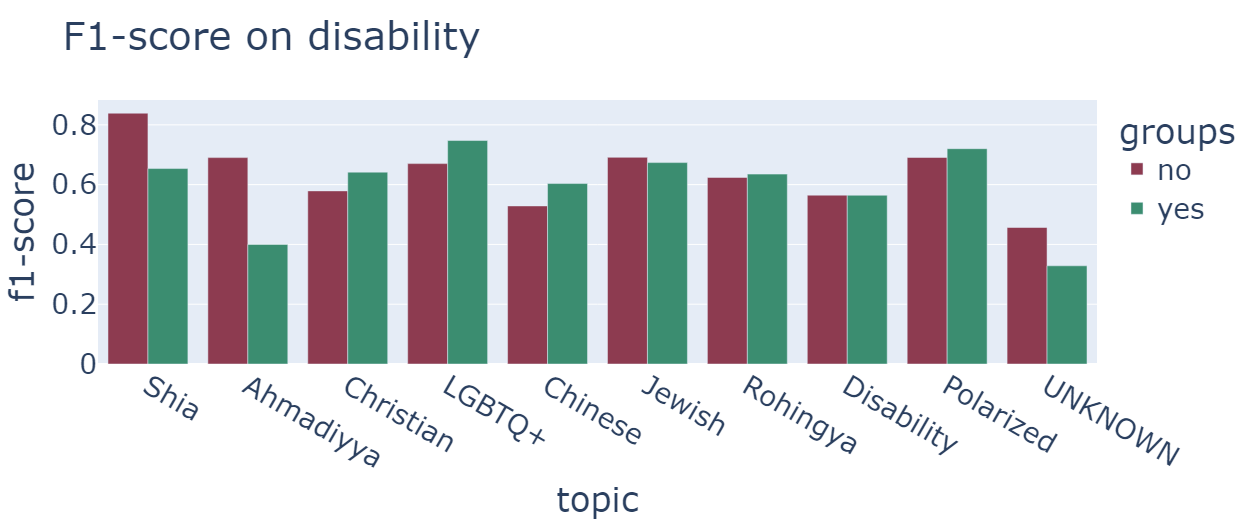}
    \label{fig:demotopic-disability}
\end{figure}
\begin{figure}[h]
    \centering
    \includegraphics[width=1\textwidth]{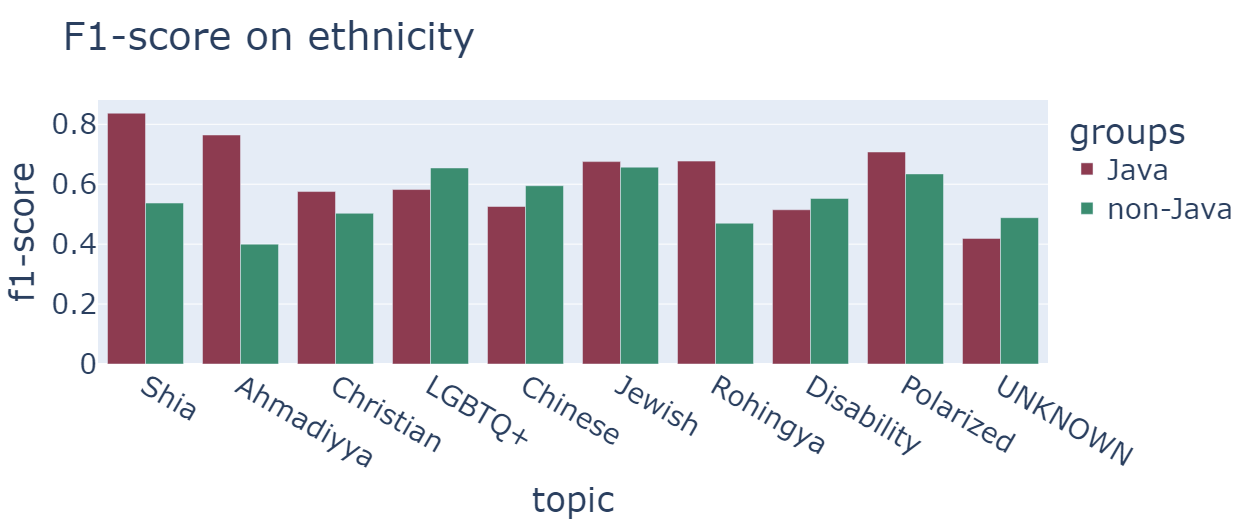}
    \label{fig:demotopic-ethnicity}
\end{figure}

\newpage
