# Supplementary material for: A Multi-Labeled Dataset for Indonesian Discourse: Examining Toxicity, Polarization, and Demographics Information
Source: arXiv:2503.00417 source file (2025-03-01)
Supplement: Supplementary file 6 [file main_annotation_process.tex]

%\section{Flow of Main Annotation Phase}
%\label{sec:mainanot}
%Figure \ref{fig:main-annotation-process} shows the main annotation process.

%\begin{figure*}[h!]
%    \centering
%    \includegraphics[width=1\textwidth]{content/images/main_phase.drawio.png}
%    \caption{Flow of main annotation procedure of an annotator.}  
%    \label{fig:main-annotation-process}
%\end{figure*}
