# Supplementary material for: A Multi-Labeled Dataset for Indonesian Discourse: Examining Toxicity, Polarization, and Demographics Information
Source: arXiv:2503.00417 source file (2025-03-01)
Supplement: Supplementary file 7 [file synthetic-gen-prompt.tex]

\section{Prompt for Synthetic Text Generation using gpt-3.5-turbo}
\label{app:synthetic-gen-prompt}
To generate synthetic data from gpt-3.5-turbo to help increase model performance for various binary classification task, we utilize the prompt visualized in Figure \ref{fig:synth-gen}

\begin{figure}[h]
    \centering
    \includegraphics[width=0.5\textwidth]{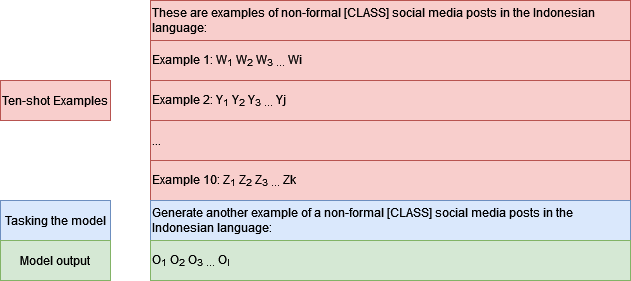}
    \caption{The template we use to prompt gpt-3.5-turbo through ten-shot prompting.}  
    \label{fig:synth-gen}
    \vspace{-15pt}
\end{figure}
