# Supplementary material for: A Multi-Labeled Dataset for Indonesian Discourse: Examining Toxicity, Polarization, and Demographics Information
Source: arXiv:2503.00417 source file (2025-03-01)
Supplement: Supplementary file 8 [file topic_keywords_mapping.tex]

\section{Mapping of \textbf{Keywords-to-Topics}}
\label{sec:mapping_topics}

\begin{compactitem}
\item \textbf{Shia} : shia, syia, syiah
\item \textbf{Ahmadiyya} : ahmadiya, ahmadiyah, ahmadiyya, ahmadiyyah
\item \textbf{Christian} : anti christ, anti kristus, anti-christ, kris10, kristen, kr1st3n, katolik, khatolik
\item \textbf{LGBTQ}+ : bisex, bisexual, eljibiti, gay, lesbian, lesbong, lgbt, lgbtq+, lghdtv+, queer, transgender
\item \textbf{Chinese} : china, chindo, chinese, cina, cindo, cokin, tionghoa
\item \textbf{Jewish} : is ra hell, israel, jew, jewish, joo, netanyahu, netanhayu, setanyahu, yahudi, zionis, bangsa pengecut
\item \textbf{Rohingya} : rohingya, imigran, pengungsi
\item \textbf{Disability} : odgj, idiot, autis, bisu, budek, buta, cacat, gangguan jiwa, gangguan mental, gila, ogdj, sinting, orang gila, orgil, sakit jiwa, tuli, tuna netra, tuna rungu, conge, gendut
\end{compactitem}
